# Supplementary material for: Spin-s Dicke states and their preparation
Source: arXiv:2402.03233 source file (2024-08-18)
Supplement: Supplementary file 1 [file s=1.5_Dicke_arxiv.pdf]

# Spin-3/2 Dicke states

```
try:
    import cirq
except ImportError:
    print("installing cirq...")
    !pip install --quiet cirq
    import cirq

    print("installed cirq.")
```

```
installing cirq...
     ━━━━━━━━━━━━━━━━━━━━━━━━━━━━━━━━━━━━━━━━ 1.8/1.8 MB 11.7 MB/s eta 0:00:00
     ━━━━━━━━━━━━━━━━━━━━━━━━━━━━━━━━━━━━━━━━ 143.1/143.1 kB 7.0 MB/s eta 0:00:00
     ━━━━━━━━━━━━━━━━━━━━━━━━━━━━━━━━━━━━━━━━ 598.8/598.8 kB 4.6 MB/s eta 0:00:00
     ━━━━━━━━━━━━━━━━━━━━━━━━━━━━━━━━━━━━━━━━ 60.9/60.9 kB 1.1 MB/s eta 0:00:00
     ━━━━━━━━━━━━━━━━━━━━━━━━━━━━━━━━━━━━━━━━ 66.2/66.2 kB 1.3 MB/s eta 0:00:00
     ━━━━━━━━━━━━━━━━━━━━━━━━━━━━━━━━━━━━━━━━ 596.5/596.5 kB 9.0 MB/s eta 0:00:00
     ━━━━━━━━━━━━━━━━━━━━━━━━━━━━━━━━━━━━━━━━ 223.8/223.8 kB 3.0 MB/s eta 0:00:00
     ━━━━━━━━━━━━━━━━━━━━━━━━━━━━━━━━━━━━━━━━ 229.9/229.9 kB 12.0 MB/s eta 0:00:00
  Preparing metadata (setup.py) ... done
     ━━━━━━━━━━━━━━━━━━━━━━━━━━━━━━━━━━━━━━━━ 151.7/151.7 kB 10.0 MB/s eta 0:00:00
     ━━━━━━━━━━━━━━━━━━━━━━━━━━━━━━━━━━━━━━━━ 45.6/45.6 kB 4.1 MB/s eta 0:00:00
  Preparing metadata (setup.py) ... done
     ━━━━━━━━━━━━━━━━━━━━━━━━━━━━━━━━━━━━━━━━ 1.6/1.6 MB 31.6 MB/s eta 0:00:00
     ━━━━━━━━━━━━━━━━━━━━━━━━━━━━━━━━━━━━━━━━ 151.7/151.7 kB 20.3 MB/s eta 0:00:00
     ━━━━━━━━━━━━━━━━━━━━━━━━━━━━━━━━━━━━━━━━ 151.7/151.7 kB 19.0 MB/s eta 0:00:00
     ━━━━━━━━━━━━━━━━━━━━━━━━━━━━━━━━━━━━━━━━ 147.4/147.4 kB 17.9 MB/s eta 0:00:00
     ━━━━━━━━━━━━━━━━━━━━━━━━━━━━━━━━━━━━━━━━ 147.4/147.4 kB 19.1 MB/s eta 0:00:00
     ━━━━━━━━━━━━━━━━━━━━━━━━━━━━━━━━━━━━━━━━ 147.4/147.4 kB 15.6 MB/s eta 0:00:00
     ━━━━━━━━━━━━━━━━━━━━━━━━━━━━━━━━━━━━━━━━ 142.7/142.7 kB 18.1 MB/s eta 0:00:00
     ━━━━━━━━━━━━━━━━━━━━━━━━━━━━━━━━━━━━━━━━ 85.5/85.5 kB 12.4 MB/s eta 0:00:00
     ━━━━━━━━━━━━━━━━━━━━━━━━━━━━━━━━━━━━━━━━ 85.1/85.1 kB 10.2 MB/s eta 0:00:00
     ━━━━━━━━━━━━━━━━━━━━━━━━━━━━━━━━━━━━━━━━ 84.7/84.7 kB 11.4 MB/s eta 0:00:00
     ━━━━━━━━━━━━━━━━━━━━━━━━━━━━━━━━━━━━━━━━ 83.6/83.6 kB 11.7 MB/s eta 0:00:00
     ━━━━━━━━━━━━━━━━━━━━━━━━━━━━━━━━━━━━━━━━ 83.3/83.3 kB 11.6 MB/s eta 0:00:00
     ━━━━━━━━━━━━━━━━━━━━━━━━━━━━━━━━━━━━━━━━ 83.4/83.4 kB 9.6 MB/s eta 0:00:00
     ━━━━━━━━━━━━━━━━━━━━━━━━━━━━━━━━━━━━━━━━ 83.2/83.2 kB 10.3 MB/s eta 0:00:00
     ━━━━━━━━━━━━━━━━━━━━━━━━━━━━━━━━━━━━━━━━ 82.5/82.5 kB 11.3 MB/s eta 0:00:00
     ━━━━━━━━━━━━━━━━━━━━━━━━━━━━━━━━━━━━━━━━ 81.0/81.0 kB 10.3 MB/s eta 0:00:00
     ━━━━━━━━━━━━━━━━━━━━━━━━━━━━━━━━━━━━━━━━ 81.0/81.0 kB 11.4 MB/s eta 0:00:00
     ━━━━━━━━━━━━━━━━━━━━━━━━━━━━━━━━━━━━━━━━ 80.8/80.8 kB 10.7 MB/s eta 0:00:00
     ━━━━━━━━━━━━━━━━━━━━━━━━━━━━━━━━━━━━━━━━ 80.7/80.7 kB 11.5 MB/s eta 0:00:00
     ━━━━━━━━━━━━━━━━━━━━━━━━━━━━━━━━━━━━━━━━ 81.5/81.5 kB 10.9 MB/s eta 0:00:00
     ━━━━━━━━━━━━━━━━━━━━━━━━━━━━━━━━━━━━━━━━ 90.4/90.4 kB 12.6 MB/s eta 0:00:00
     ━━━━━━━━━━━━━━━━━━━━━━━━━━━━━━━━━━━━━━━━ 117.7/117.7 kB 16.0 MB/s eta 0:00:00
     ━━━━━━━━━━━━━━━━━━━━━━━━━━━━━━━━━━━━━━━━ 60.6/60.6 kB 8.1 MB/s eta 0:00:00
     ━━━━━━━━━━━━━━━━━━━━━━━━━━━━━━━━━━━━━━━━ 71.5/71.5 kB 10.4 MB/s eta 0:00:00
     ━━━━━━━━━━━━━━━━━━━━━━━━━━━━━━━━━━━━━━━━ 1.7/1.7 MB 37.8 MB/s eta 0:00:00
     ━━━━━━━━━━━━━━━━━━━━━━━━━━━━━━━━━━━━━━━━ 116.4/116.4 kB 16.3 MB/s eta 0:00:00
     ━━━━━━━━━━━━━━━━━━━━━━━━━━━━━━━━━━━━━━━━ 69.6/69.6 kB 9.8 MB/s eta 0:00:00
     ━━━━━━━━━━━━━━━━━━━━━━━━━━━━━━━━━━━━━━━━ 526.7/526.7 kB 40.0 MB/s eta 0:00:00
     ━━━━━━━━━━━━━━━━━━━━━━━━━━━━━━━━━━━━━━━━ 58.3/58.3 kB 8.5 MB/s eta 0:00:00
  Building wheel for lark (setup.py) ... done
  Building wheel for rpcq (setup.py) ... done
ERROR: pip's dependency resolver does not currently take into account all the packages that are installed. This be
lida 0.0.10 requires fastapi, which is not installed.
lida 0.0.10 requires kaleido, which is not installed.
lida 0.0.10 requires python-multipart, which is not installed.
lida 0.0.10 requires uvicorn, which is not installed.
referencing 0.32.1 requires attrs>=22.2.0, but you have attrs 21.4.0 which is incompatible.
installed cirq.
```

## Basic $d = 4$ gates

```
import numpy as np


import math


simulator = cirq.Simulator()


class X01(cirq.Gate):

  def _qid_shape_(self):
    return (4,)

  def _unitary_(self):
    return np.array([[0, 1, 0, 0],
                    [1, 0, 0, 0],
                    [0, 0, 1, 0],
                     [0, 0, 0, 1]])

  def _circuit_diagram_info_(self, args):
        return 'X01'

class X02(cirq.Gate):

  def _qid_shape_(self):
    return (4,)

  def _unitary_(self):
    return np.array([[0, 0, 1, 0],
                    [0, 1, 0, 0],
                    [1, 0, 0, 0],
                     [0, 0, 0, 1]])

  def _circuit_diagram_info_(self, args):
        return 'X02'

class X03(cirq.Gate):

  def _qid_shape_(self):
    return (4,)

  def _unitary_(self):
    return np.array([[0, 0, 0, 1],
                    [0, 1, 0, 0],
                    [0, 0, 1, 0],
                     [1, 0, 0, 0]])

  def _circuit_diagram_info_(self, args):
        return 'X03'

class X12(cirq.Gate):

  def _qid_shape_(self):
    return (4,)

  def _unitary_(self):
    return np.array([[1, 0, 0, 0],
                    [0, 0, 1, 0],
                    [0, 1, 0, 0],
                     [0, 0, 0, 1]])

  def _circuit_diagram_info_(self, args):
```

```
            return 'X12'

    class X13(cirq.Gate):

      def _qid_shape_(self):
        return (4,)

      def _unitary_(self):
        return np.array([[1, 0, 0, 0],
                        [0, 0, 0, 1],
                        [0, 0, 1, 0],
                         [0, 1, 0, 0]])

      def _circuit_diagram_info_(self, args):
            return 'X13'

    class X23(cirq.Gate):

      def _qid_shape_(self):
        return (4,)

      def _unitary_(self):
        return np.array([[1, 0, 0, 0],
                        [0, 1, 0, 0],
                        [0, 0, 0, 1],
                         [0, 0, 1, 0]])

      def _circuit_diagram_info_(self, args):
            return 'X23'

    class R01(cirq.Gate):

      def __init__(self, theta):
            super(R01, self)
            self.theta = theta

      def _qid_shape_(self):
        return (4,)

      def _unitary_(self):
        return np.array([[np.cos(self.theta/2), -np.sin(self.theta/2), 0, 0],
                        [np.sin(self.theta/2), np.cos(self.theta/2), 0, 0],
                        [0, 0, 1, 0],
                         [0, 0, 0, 1]])

      def _circuit_diagram_info_(self, args):
            return f"R01({self.theta})"

    class R02(cirq.Gate):

      def __init__(self, theta):
            super(R02, self)
            self.theta = theta

      def _qid_shape_(self):
        return (4,)

      def _unitary_(self):
        return np.array([[np.cos(self.theta/2), 0, -np.sin(self.theta/2), 0],
                         [0, 1, 0, 0],
                         [np.sin(self.theta/2), 0, np.cos(self.theta/2), 0],
                         [0, 0, 0, 1] ])

      def _circuit_diagram_info_(self, args):
            return f"R02({self.theta})"
```

```
class R12(cirq.Gate):

  def __init__(self, theta):
      super(R12, self)
      self.theta = theta

  def _qid_shape_(self):
    return (4,)

  def _unitary_(self):
    return np.array([[1, 0, 0, 0],
                     [0, np.cos(self.theta/2), -np.sin(self.theta/2), 0],
                     [0, np.sin(self.theta/2), np.cos(self.theta/2), 0],
                     [0, 0, 0, 1] ])

  def _circuit_diagram_info_(self, args):
      return f"R12({self.theta})"


class R23(cirq.Gate):

  def __init__(self, theta):
      super(R23, self)
      self.theta = theta

  def _qid_shape_(self):
    return (4,)

  def _unitary_(self):
    return np.array([[1, 0, 0, 0],
                     [0, 1, 0, 0],
                     [0, 0, np.cos(self.theta/2), -np.sin(self.theta/2)],
                     [0, 0, np.sin(self.theta/2), np.cos(self.theta/2)] ])

  def _circuit_diagram_info_(self, args):
      return f"R23({self.theta})"


class myid(cirq.Gate):

  def _qid_shape_(self):
    return (4,)

  def _unitary_(self):
    return np.array([[1, 0, 0, 0],
                    [0, 1, 0, 0],
                    [0, 0, 1, 0],
                    [0, 0, 0, 1]])

  def _circuit_diagram_info_(self, args):
      return 'id'
```

## $T_{m,k} \qquad (1 \leq k \leq 3n-1)$

```
def cc(n,k,j):
  s=3/2
  ss=round(2*s)
  num=math.comb(k,j)*math.factorial(ss)*math.factorial(ss*n-ss)\
  *math.factorial(ss*n-k)
  denom=math.factorial(ss-j)*math.factorial(ss*n)\
  *math.factorial(ss*n+j-k-ss)
  return math.sqrt(num/denom)
```

```
# 0

# k = 3l , 2 \le l \le m-1 , m \ge 3
def t_gate0_a(qr,m,l):
  """Gives generator"""
  # l=k/3
  k=3*l
  cx01 = cirq.ControlledGate(X01(),num_controls=1, control_values=(3,),\
                             control_qid_shape=(4,))
  cx12 = cirq.ControlledGate(X12(),num_controls=1, control_values=(2,),\
                             control_qid_shape=(4,))
  cx23 = cirq.ControlledGate(X23(),num_controls=1, control_values=(1,),\
                             control_qid_shape=(4,))

  theta1=2*np.arccos(cc(m,k,3))
  theta2=2*np.arccos(cc(m,k,2)/(np.tan(theta1/2)*cc(m,k,3)))
  theta3=2*np.arctan(cc(m,k,0)/cc(m,k,1))

  ccr23 = cirq.ControlledGate(R23(-theta1),num_controls=2, \
                              control_values=((1,),(3,)),\
                              control_qid_shape=(4,4))
  ccr12 = cirq.ControlledGate(R12(-theta2),num_controls=2, \
                              control_values=((2,),(3,)),\
                              control_qid_shape=(4,4))
  ccr01 = cirq.ControlledGate(R01(-theta3),num_controls=2, \
                              control_values=((3,),(3,)),\
                              control_qid_shape=(4,4))

  yield cx01(qr[0],qr[l])
  yield ccr23(qr[l],qr[l-1],qr[0])
  yield cx01(qr[0],qr[l])

  yield cx12(qr[0],qr[l])
  yield ccr12(qr[l],qr[l-1],qr[0])
  yield cx12(qr[0],qr[l])

  yield cx23(qr[0],qr[l])
  yield ccr01(qr[l],qr[l-1],qr[0])
  yield cx23(qr[0],qr[l])


# k = 3l , l=1 , m \ge 2
def t_gate0_b(qr,m,l):
  """Gives generator"""
  # l=1
  k=3*l
  cx01 = cirq.ControlledGate(X01(),num_controls=1, control_values=(3,),\
                             control_qid_shape=(4,))
  cx12 = cirq.ControlledGate(X12(),num_controls=1, control_values=(2,),\
                             control_qid_shape=(4,))
  cx23 = cirq.ControlledGate(X23(),num_controls=1, control_values=(1,),\
                             control_qid_shape=(4,))

  theta1=2*np.arccos(cc(m,k,3))
  theta2=2*np.arccos(cc(m,k,2)/(np.tan(theta1/2)*cc(m,k,3)))
  theta3=2*np.arctan(cc(m,k,0)/cc(m,k,1))

  cr23 = cirq.ControlledGate(R23(-theta1),num_controls=1, control_values=(1,),\
                             control_qid_shape=(4,))
  cr12 = cirq.ControlledGate(R12(-theta2),num_controls=1, control_values=(2,),\
                             control_qid_shape=(4,))
  cr01 = cirq.ControlledGate(R01(-theta3),num_controls=1, control_values=(3,),\
                             control_qid_shape=(4,))

  yield cx01(qr[0],qr[l])
  yield cr23(qr[l],qr[0])
```

```
    yield cx01(qr[0],qr[l])

    yield cx12(qr[0],qr[l])
    yield cr12(qr[l],qr[0])
    yield cx12(qr[0],qr[l])

    yield cx23(qr[0],qr[l])
    yield cr01(qr[l],qr[0])
    yield cx23(qr[0],qr[l])

  # 1

  # k = 3l+1 , 2 \le l \le m-2 , m \ge 4
  def t_gate1_a(qr,m,l):
    """Gives generator"""
    k=3*l+1
    cx01 = cirq.ControlledGate(X01(),num_controls=1, control_values=(1,),\
                               control_qid_shape=(4,))
    cx12 = cirq.ControlledGate(X12(),num_controls=1, control_values=(3,),\
                               control_qid_shape=(4,))
    cx23 = cirq.ControlledGate(X23(),num_controls=1, control_values=(2,),\
                               control_qid_shape=(4,))

    theta1=2*np.arccos(cc(m,k,3))
    theta2=2*np.arccos(cc(m,k,2)/(np.tan(theta1/2)*cc(m,k,3)))
    theta3=2*np.arctan(cc(m,k,0)/cc(m,k,1))

    ccr23 = cirq.ControlledGate(R23(-theta1),num_controls=2, \
                                control_values=((2,),(3,)),\
                                control_qid_shape=(4,4))
    ccr12 = cirq.ControlledGate(R12(-theta2),num_controls=2, \
                                control_values=((3,),(3,)),\
                                control_qid_shape=(4,4))
    ccr01 = cirq.ControlledGate(R01(-theta3),num_controls=2, \
                                control_values=((1,),(3,)),\
                                control_qid_shape=(4,4))

    yield cx12(qr[0],qr[l])
    yield ccr23(qr[l],qr[l-1],qr[0])
    yield cx12(qr[0],qr[l])

    yield cx23(qr[0],qr[l])
    yield ccr12(qr[l],qr[l-1],qr[0])
    yield cx23(qr[0],qr[l])

    yield cx01(qr[0],qr[l+1])
    yield ccr01(qr[l+1],qr[l],qr[0])
    yield cx01(qr[0],qr[l+1])


  # k = 3l+1 , l= m-1 , m \ge 3
  def t_gate1_b(qr,m,l):
    """Gives generator"""
    # l=m-1
    k=3*l+1
    cx12 = cirq.ControlledGate(X12(),num_controls=1, control_values=(3,),\
                               control_qid_shape=(4,))
    cx23 = cirq.ControlledGate(X23(),num_controls=1, control_values=(2,),\
                               control_qid_shape=(4,))

    theta1=2*np.arccos(cc(m,k,3))
    theta2=2*np.arccos(cc(m,k,2)/(np.tan(theta1/2)*cc(m,k,3)))

    ccr23 = cirq.ControlledGate(R23(-theta1),num_controls=2, \
                                control_values=((2,),(3,)),\
                                control_qid_shape=(4,4))
```

```
    ccr12 = cirq.ControlledGate(R12(-theta2),num_controls=2, \
                                control_values=((3,),(3,)),\
                                control_qid_shape=(4,4))

    yield cx12(qr[0],qr[l])
    yield ccr23(qr[l],qr[l-1],qr[0])
    yield cx12(qr[0],qr[l])

    yield cx23(qr[0],qr[l])
    yield ccr12(qr[l],qr[l-1],qr[0])
    yield cx23(qr[0],qr[l])


  # k = 3l+1 , l=1, m=2
  def t_gate1_c(qr,m,l):
    """Gives generator"""
    # m=2
    # l=1
    k=3*l+1
    cx12 = cirq.ControlledGate(X12(),num_controls=1, control_values=(3,),\
                               control_qid_shape=(4,))
    cx23 = cirq.ControlledGate(X23(),num_controls=1, control_values=(2,),\
                               control_qid_shape=(4,))

    theta1=2*np.arccos(cc(m,k,3))
    theta2=2*np.arccos(cc(m,k,2)/(np.tan(theta1/2)*cc(m,k,3)))

    cr23 = cirq.ControlledGate(R23(-theta1),num_controls=1, control_values=(2,),\
                               control_qid_shape=(4,))
    cr12 = cirq.ControlledGate(R12(-theta2),num_controls=1, control_values=(3,),\
                               control_qid_shape=(4,))

    yield cx12(qr[0],qr[l])
    yield cr23(qr[l],qr[0])
    yield cx12(qr[0],qr[l])

    yield cx23(qr[0],qr[l])
    yield cr12(qr[l],qr[0])
    yield cx23(qr[0],qr[l])


  # k = 3l+1 , l=1 , m \ge 3
  def t_gate1_d(qr,m,l):
    """Gives generator"""
    # l=1
    k=3*l+1

    cx01 = cirq.ControlledGate(X01(),num_controls=1, control_values=(1,),\
                               control_qid_shape=(4,))
    cx12 = cirq.ControlledGate(X12(),num_controls=1, control_values=(3,),\
                               control_qid_shape=(4,))
    cx23 = cirq.ControlledGate(X23(),num_controls=1, control_values=(2,),\
                               control_qid_shape=(4,))


    theta1=2*np.arccos(cc(m,k,3))
    theta2=2*np.arccos(cc(m,k,2)/(np.tan(theta1/2)*cc(m,k,3)))
    theta3=2*np.arctan(cc(m,k,0)/cc(m,k,1))

    cr23 = cirq.ControlledGate(R23(-theta1),num_controls=1, control_values=(2,),\
                               control_qid_shape=(4,))
    cr12 = cirq.ControlledGate(R12(-theta2),num_controls=1, control_values=(3,),\
                               control_qid_shape=(4,))
    ccr01 = cirq.ControlledGate(R01(-theta3),num_controls=2, \
                                control_values=((1,),(3,)),\
                                control_qid_shape=(4,4))
```

```
    yield cx12(qr[0],qr[l])
    yield cr23(qr[l],qr[0])
    yield cx12(qr[0],qr[l])

    yield cx23(qr[0],qr[l])
    yield cr12(qr[l],qr[0])
    yield cx23(qr[0],qr[l])

    yield cx01(qr[0],qr[l+1])
    yield ccr01(qr[l+1],qr[l],qr[0])
    yield cx01(qr[0],qr[l+1])


  # k = 3l+1,  l=0 , m \ge 2
  def t_gate1_e(qr,m,l):
    """Gives generator"""
    # l=0
    k=3*l+1

    cx01 = cirq.ControlledGate(X01(),num_controls=1, control_values=(1,),\
                               control_qid_shape=(4,))

    theta3=2*np.arctan(cc(m,k,0)/cc(m,k,1))

    cr01 = cirq.ControlledGate(R01(-theta3),num_controls=1, control_values=(1,),\
                               control_qid_shape=(4,))

    yield cx01(qr[0],qr[l+1])
    yield cr01(qr[l+1],qr[0])
    yield cx01(qr[0],qr[l+1])

  # 2

  # k = 3l+2 , 2 \le l \le m-2 , m \ge 4
  def t_gate2_a(qr,m,l):
    """Gives generator"""
    k=3*l+2

    cx01 = cirq.ControlledGate(X01(),num_controls=1, control_values=(2,),\
                               control_qid_shape=(4,))
    cx12 = cirq.ControlledGate(X12(),num_controls=1, control_values=(1,),\
                               control_qid_shape=(4,))
    cx23 = cirq.ControlledGate(X23(),num_controls=1, control_values=(3,),\
                               control_qid_shape=(4,))

    theta1=2*np.arccos(cc(m,k,3))
    theta2=2*np.arccos(cc(m,k,2)/(np.tan(theta1/2)*cc(m,k,3)))
    theta3=2*np.arctan(cc(m,k,0)/cc(m,k,1))

    ccr23 = cirq.ControlledGate(R23(-theta1),num_controls=2, \
                                control_values=((3,),(3,)),\
                                control_qid_shape=(4,4))
    ccr12 = cirq.ControlledGate(R12(-theta2),num_controls=2, \
                                control_values=((1,),(3,)),\
                                control_qid_shape=(4,4))
    ccr01 = cirq.ControlledGate(R01(-theta3),num_controls=2, \
                                control_values=((2,),(3,)),\
                                control_qid_shape=(4,4))

    yield cx23(qr[0],qr[l])
    yield ccr23(qr[l],qr[l-1],qr[0])
    yield cx23(qr[0],qr[l])

    yield cx01(qr[0],qr[l+1])
    yield ccr12(qr[l+1],qr[l],qr[0])
```

```
    yield cx01(qr[0],qr[l+1])

    yield cx12(qr[0],qr[l+1])
    yield ccr01(qr[l+1],qr[l],qr[0])
    yield cx12(qr[0],qr[l+1])


  # k = 3l+2 , l= m-1 , m \ge 3
  def t_gate2_b(qr,m,l):
    """Gives generator"""
    # l=m-1
    k=3*l+2

    cx23 = cirq.ControlledGate(X23(),num_controls=1, control_values=(3,),\
                               control_qid_shape=(4,))

    theta1=2*np.arccos(cc(m,k,3))

    ccr23 = cirq.ControlledGate(R23(-theta1),num_controls=2, \
                                control_values=((3,),(3,)),\
                                control_qid_shape=(4,4))

    yield cx23(qr[0],qr[l])
    yield ccr23(qr[l],qr[l-1],qr[0])
    yield cx23(qr[0],qr[l])


  # k = 3l+2 , l=1, m=2
  def t_gate2_c(qr,m,l):
    """Gives generator"""
    # m=2
    # l=1
    k=3*l+2

    cx23 = cirq.ControlledGate(X23(),num_controls=1, control_values=(3,),\
                               control_qid_shape=(4,))

    theta1=2*np.arccos(cc(m,k,3))

    cr23 = cirq.ControlledGate(R23(-theta1),num_controls=1, control_values=(3,),\
                               control_qid_shape=(4,))

    yield cx23(qr[0],qr[l])
    yield cr23(qr[l],qr[0])
    yield cx23(qr[0],qr[l])


  # k = 3l+2 , l=1 , m \ge 3
  def t_gate2_d(qr,m,l):
    """Gives generator"""
    # l=1
    k=3*l+2

    cx01 = cirq.ControlledGate(X01(),num_controls=1, control_values=(2,),\
                               control_qid_shape=(4,))
    cx12 = cirq.ControlledGate(X12(),num_controls=1, control_values=(1,),\
                               control_qid_shape=(4,))
    cx23 = cirq.ControlledGate(X23(),num_controls=1, control_values=(3,),\
                               control_qid_shape=(4,))


    theta1=2*np.arccos(cc(m,k,3))
    theta2=2*np.arccos(cc(m,k,2)/(np.tan(theta1/2)*cc(m,k,3)))
    theta3=2*np.arctan(cc(m,k,0)/cc(m,k,1))

    cr23 = cirq.ControlledGate(R23(-theta1),num_controls=1, control_values=(3,),\
```

```
                             control_qid_shape=(4,))
  ccr12 = cirq.ControlledGate(R12(-theta2),num_controls=2,\
                              control_values=((1,),(3,)),\
                             control_qid_shape=(4,4))
  ccr01 = cirq.ControlledGate(R01(-theta3),num_controls=2, \
                              control_values=((2,),(3,)),\
                              control_qid_shape=(4,4))

  yield cx23(qr[0],qr[l])
  yield cr23(qr[l],qr[0])
  yield cx23(qr[0],qr[l])

  yield cx01(qr[0],qr[l+1])
  yield ccr12(qr[l+1],qr[l],qr[0])
  yield cx01(qr[0],qr[l+1])

  yield cx01(qr[0],qr[l+1])
  yield ccr01(qr[l+1],qr[l],qr[0])
  yield cx01(qr[0],qr[l+1])


# k = 3l+2,  l=0 , m \ge 2
def t_gate2_e(qr,m,l):
  """Gives generator"""
  # l=0
  k=3*l+2

  cx01 = cirq.ControlledGate(X01(),num_controls=1, control_values=(2,),\
                             control_qid_shape=(4,))
  cx12 = cirq.ControlledGate(X12(),num_controls=1, control_values=(1,),\
                             control_qid_shape=(4,))

  #theta1=2*np.arccos(cc(m,k,3))
  #special case, since here cc(m,k,3) == 0
  theta2=2*np.arccos(cc(m,k,2))
  theta3=2*np.arctan(cc(m,k,0)/cc(m,k,1))

  cr12 = cirq.ControlledGate(R12(-theta2),num_controls=1, control_values=(1,),\
                             control_qid_shape=(4,))
  cr01 = cirq.ControlledGate(R01(-theta3),num_controls=1, control_values=(2,),\
                             control_qid_shape=(4,))


  yield cx01(qr[0],qr[l+1])
  yield cr12(qr[l+1],qr[0])
  yield cx01(qr[0],qr[l+1])

  yield cx12(qr[0],qr[l+1])
  yield cr01(qr[l+1],qr[0])
  yield cx12(qr[0],qr[l+1])



def t_gate(qr,m,k):
  l=round(np.floor(k/3))
  if k==3*l:
     mycase=0
  elif k==3*l+1:
     mycase=1
  elif k==3*l+2:
     mycase=2

  #mycase=0

  if mycase==0 and 2 <= l <= m-1 and m>=3:
    yield t_gate0_a(qr,m,l)
```

```
    elif mycase==0 and l==1 and m>=2:
      yield t_gate0_b(qr,m,l)

    #mycase=1

    elif mycase==1 and 2 <= l <= m-2 and m>=4:
      yield t_gate1_a(qr,m,l)

    elif mycase==1 and l== m-1 and m>=3:
      yield t_gate1_b(qr,m,l)

    elif mycase==1 and l== 1 and m==2:
      yield t_gate1_c(qr,m,l)

    elif mycase==1 and l== 1 and m>=3:
      yield t_gate1_d(qr,m,l)

    elif mycase==1 and l== 0 and m>=2:
      yield t_gate1_e(qr,m,l)

    #mycase=2

    elif mycase==2 and 2 <= l <= m-2 and m>=4:
      yield t_gate2_a(qr,m,l)

    elif mycase==2 and l== m-1 and m>=3:
      yield t_gate2_b(qr,m,l)

    elif mycase==2 and l== 1 and m==2:
      yield t_gate2_c(qr,m,l)

    elif mycase==2 and l== 1 and m>=3:
      yield t_gate2_d(qr,m,l)

    elif mycase==2 and l== 0 and m>=2:
      yield t_gate2_e(qr,m,l)
```

## NOT simplified

```
def W(qr,m):
  for k in range(1,3*m):
    yield t_gate(qr,m,k)

#W \otimes identity:
def WW(qr,n,m):
  yield W(qr[n-m:n],m)

def UU(qr,n):
  for m in reversed(range(2,n+1)):
    yield WW(qr,n,m)

def spin32Dicke(qr,n,k):
  """Gives generator"""
  # 0 < k < 3n
  # initial state
  l=round(np.floor(k/3))
  if k==3*l:
    for j in range(l):
      yield X03()(qr[j])

  elif k==3*l+1:
    for j in range(l):
      yield X03()(qr[j])
    yield X01()(qr[l])

  elif k==3*l+2:
    for j in range(l):
      yield X03()(qr[j])
    yield X02()(qr[l])

  # apply Dicke operator
  yield UU(qr,n)
```

## n=2

```
n=2
k=1
# 0 < k < 3n
qr = cirq.LineQid.range(n, dimension=4)
test=cirq.Circuit(spin32Dicke(qr,n,k))
#print(test)
result = simulator.simulate(test)
print(cirq.dirac_notation(result.final_state_vector, qid_shape=(4,)*n))
```

```
0.71|01⟩ + 0.71|10⟩
```

```
n=2
k=2
# 0 < k < 3n
qr = cirq.LineQid.range(n, dimension=4)
test=cirq.Circuit(spin32Dicke(qr,n,k))
#print(test)
result = simulator.simulate(test)
print(cirq.dirac_notation(result.final_state_vector, qid_shape=(4,)*n))
```

```
0.45|02⟩ + 0.77|11⟩ + 0.45|20⟩
```

```
n=2
k=3
# 0 < k < 3n
qr = cirq.LineQid.range(n, dimension=4)
test=cirq.Circuit(spin32Dicke(qr,n,k))
#print(test)
result = simulator.simulate(test)
print(cirq.dirac_notation(result.final_state_vector, qid_shape=(4,)*n))
```

```
0.22|03⟩ + 0.67|12⟩ + 0.67|21⟩ + 0.22|30⟩
```

```
n=2
k=4
# 0 < k < 3n
qr = cirq.LineQid.range(n, dimension=4)
test=cirq.Circuit(spin32Dicke(qr,n,k))
#print(test)
result = simulator.simulate(test)
print(cirq.dirac_notation(result.final_state_vector, qid_shape=(4,)*n))
```

```
0.45|13⟩ + 0.77|22⟩ + 0.45|31⟩
```

```
n=2
k=5
# 0 < k < 3n
qr = cirq.LineQid.range(n, dimension=4)
test=cirq.Circuit(spin32Dicke(qr,n,k))
#print(test)
result = simulator.simulate(test)
print(cirq.dirac_notation(result.final_state_vector, qid_shape=(4,)*n))
```

```
0.71|23⟩ + 0.71|32⟩
```

## n=3

```
n=3
k=1
# 0 < k < 3n
qr = cirq.LineQid.range(n, dimension=4)
test=cirq.Circuit(spin32Dicke(qr,n,k))
#print(test)
result = simulator.simulate(test)
print(cirq.dirac_notation(result.final_state_vector, qid_shape=(4,)*n))
```

```
0.58|001⟩ + 0.58|010⟩ + 0.58|100⟩
```

```
n=3
k=2
# 0 < k < 3n
qr = cirq.LineQid.range(n, dimension=4)
test=cirq.Circuit(spin32Dicke(qr,n,k))
#print(test)
result = simulator.simulate(test)
print(cirq.dirac_notation(result.final_state_vector, qid_shape=(4,)*n))
```

```
0.29|002⟩ + 0.5|011⟩ + 0.29|020⟩ + 0.5|101⟩ + 0.5|110⟩ + 0.29|200⟩
```

```
n=3
k=3
# 0 < k < 3n
qr = cirq.LineQid.range(n, dimension=4)
test=cirq.Circuit(spin32Dicke(qr,n,k))
#print(test)
result = simulator.simulate(test)
print(cirq.dirac_notation(result.final_state_vector, qid_shape=(4,)*n))
```

```
0.11|003⟩ + 0.33|012⟩ + 0.33|021⟩ + 0.11|030⟩ + 0.33|102⟩ + 0.57|111⟩ + 0.33|120⟩ + 0.33|201⟩ + 0.33|210⟩ + 0.11|300⟩
```

```
n=3
k=4
# 0 < k < 3n
qr = cirq.LineQid.range(n, dimension=4)
test=cirq.Circuit(spin32Dicke(qr,n,k))
#print(test)
result = simulator.simulate(test)
print(cirq.dirac_notation(result.final_state_vector, qid_shape=(4,)*n))
```

```
0.15|013⟩ + 0.27|022⟩ + 0.15|031⟩ + 0.15|103⟩ + 0.46|112⟩ + 0.46|121⟩ + 0.15|130⟩ + 0.27|202⟩ + 0.46|211⟩ + 0.27|220⟩
```

```
n=3
k=5
# 0 < k < 3n
qr = cirq.LineQid.range(n, dimension=4)
test=cirq.Circuit(spin32Dicke(qr,n,k))
#print(test)
result = simulator.simulate(test)
print(cirq.dirac_notation(result.final_state_vector, qid_shape=(4,)*n))
```

```
0.28|113⟩ + 0.49|122⟩ + 0.28|131⟩ + 0.15|203⟩ + 0.46|212⟩ + 0.46|221⟩ + 0.15|230⟩ + 0.15|302⟩ + 0.27|311⟩ + 0.15|320⟩
```

```
n=3
k=6
# 0 < k < 3n
qr = cirq.LineQid.range(n, dimension=4)
test=cirq.Circuit(spin32Dicke(qr,n,k))
#print(test)
result = simulator.simulate(test)
print(cirq.dirac_notation(result.final_state_vector, qid_shape=(4,)*n))
```

```
0.11|033⟩ + 0.33|123⟩ + 0.33|132⟩ + 0.33|213⟩ + 0.57|222⟩ + 0.33|231⟩ + 0.11|303⟩ + 0.33|312⟩ + 0.33|321⟩ + 0.11|330⟩
```

```
n=3
k=7
# 0 < k < 3n
qr = cirq.LineQid.range(n, dimension=4)
test=cirq.Circuit(spin32Dicke(qr,n,k))
#print(test)
result = simulator.simulate(test)
print(cirq.dirac_notation(result.final_state_vector, qid_shape=(4,)*n))
```

```
0.29|133⟩ + 0.5|223⟩ + 0.5|232⟩ + 0.29|313⟩ + 0.5|322⟩ + 0.29|331⟩
```

```
n=3
k=8
# 0 < k < 3n
qr = cirq.LineQid.range(n, dimension=4)
test=cirq.Circuit(spin32Dicke(qr,n,k))
#print(test)
result = simulator.simulate(test)
print(cirq.dirac_notation(result.final_state_vector, qid_shape=(4,)*n))
```

```
0.58|233⟩ + 0.58|323⟩ + 0.58|332⟩
```

## n=4

```
n=4
k=1
# 0 < k < 3n
qr = cirq.LineQid.range(n, dimension=4)
test=cirq.Circuit(spin32Dicke(qr,n,k))
#print(test)
result = simulator.simulate(test)
print(cirq.dirac_notation(result.final_state_vector, qid_shape=(4,)*n))
```

```
0.5|0001⟩ + 0.5|0010⟩ + 0.5|0100⟩ + 0.5|1000⟩
```

```
n=4
k=2
# 0 < k < 3n
qr = cirq.LineQid.range(n, dimension=4)
test=cirq.Circuit(spin32Dicke(qr,n,k))
#print(test)
result = simulator.simulate(test)
print(cirq.dirac_notation(result.final_state_vector, qid_shape=(4,)*n))
```

```
0.21|0002⟩ + 0.37|0011⟩ + 0.21|0020⟩ + 0.37|0101⟩ + 0.37|0110⟩ + 0.21|0200⟩ + 0.37|1001⟩ + 0.37|1010⟩ + 0.37|1100⟩ +
```

```
n=4
k=3
# 0 < k < 3n
qr = cirq.LineQid.range(n, dimension=4)
test=cirq.Circuit(spin32Dicke(qr,n,k))
#print(test)
result = simulator.simulate(test)
print(cirq.dirac_notation(result.final_state_vector, qid_shape=(4,)*n))
```

```
0.07|0003⟩ + 0.2|0012⟩ + 0.2|0021⟩ + 0.07|0030⟩ + 0.2|0102⟩ + 0.35|0111⟩ + 0.2|0120⟩ + 0.2|0201⟩ + 0.2|0210⟩ + 0.07|0
```

```
n=4
k=4
# 0 < k < 3n
qr = cirq.LineQid.range(n, dimension=4)
test=cirq.Circuit(spin32Dicke(qr,n,k))
#print(test)
result = simulator.simulate(test)
print(cirq.dirac_notation(result.final_state_vector, qid_shape=(4,)*n))
```

```
0.08|0013⟩ + 0.13|0022⟩ + 0.08|0031⟩ + 0.08|0103⟩ + 0.23|0112⟩ + 0.23|0121⟩ + 0.08|0130⟩ + 0.13|0202⟩ + 0.23|0211⟩ +
```

```
n=4
k=5
# 0 < k < 3n
qr = cirq.LineQid.range(n, dimension=4)
test=cirq.Circuit(spin32Dicke(qr,n,k))
#print(test)
result = simulator.simulate(test)
print(cirq.dirac_notation(result.final_state_vector, qid_shape=(4,)*n))
```

```
0.12|1013⟩ + 0.21|1022⟩ + 0.12|1031⟩ + 0.12|1103⟩ + 0.37|1112⟩ + 0.37|1121⟩ + 0.12|1130⟩ + 0.21|1202⟩ + 0.37|1211⟩ +
```

```
n=4
k=6
# 0 < k < 3n
qr = cirq.LineQid.range(n, dimension=4)
test=cirq.Circuit(spin32Dicke(qr,n,k))
#print(test)
result = simulator.simulate(test)
print(cirq.dirac_notation(result.final_state_vector, qid_shape=(4,)*n))
```

```
0.03|0033⟩ + 0.1|0123⟩ + 0.1|0132⟩ + 0.1|0213⟩ + 0.17|0222⟩ + 0.1|0231⟩ + 0.03|0303⟩ + 0.1|0312⟩ + 0.1|0321⟩ + 0.03|0
```

```
n=4
k=7
# 0 < k < 3n
qr = cirq.LineQid.range(n, dimension=4)
test=cirq.Circuit(spin32Dicke(qr,n,k))
#print(test)
result = simulator.simulate(test)
print(cirq.dirac_notation(result.final_state_vector, qid_shape=(4,)*n))
```

```
0.06|0133⟩ + 0.11|0223⟩ + 0.11|0232⟩ + 0.06|0313⟩ + 0.11|0322⟩ + 0.06|0331⟩ + 0.06|1033⟩ + 0.18|1123⟩ + 0.18|1132⟩ +
```

## n=5

```
n=5
k=1
# 0 < k < 3n
qr = cirq.LineQid.range(n, dimension=4)
test=cirq.Circuit(spin32Dicke(qr,n,k))
#print(test)
result = simulator.simulate(test)
print(cirq.dirac_notation(result.final_state_vector, qid_shape=(4,)*n))
```

```
0.45|00001⟩ + 0.45|00010⟩ + 0.45|00100⟩ + 0.45|01000⟩ + 0.45|10000⟩
```

```
n=5
k=2
# 0 < k < 3n
qr = cirq.LineQid.range(n, dimension=4)
test=cirq.Circuit(spin32Dicke(qr,n,k))
#print(test)
result = simulator.simulate(test)
print(cirq.dirac_notation(result.final_state_vector, qid_shape=(4,)*n))
```

```
0.17|00002⟩ + 0.29|00011⟩ + 0.17|00020⟩ + 0.29|00101⟩ + 0.29|00110⟩ + 0.17|00200⟩ + 0.29|01001⟩ + 0.29|01010⟩ + 0.29|
```

```
n=5
k=3
# 0 < k < 3n
qr = cirq.LineQid.range(n, dimension=4)
test=cirq.Circuit(spin32Dicke(qr,n,k))
#print(test)
result = simulator.simulate(test)
print(cirq.dirac_notation(result.final_state_vector, qid_shape=(4,)*n))
```

```
0.05|00003⟩ + 0.14|00012⟩ + 0.14|00021⟩ + 0.05|00030⟩ + 0.14|00102⟩ + 0.24|00111⟩ + 0.14|00120⟩ + 0.14|00201⟩ + 0.14|
```

```
n=5
k=4
# 0 < k < 3n
qr = cirq.LineQid.range(n, dimension=4)
test=cirq.Circuit(spin32Dicke(qr,n,k))
#print(test)
result = simulator.simulate(test)
print(cirq.dirac_notation(result.final_state_vector, qid_shape=(4,)*n))
```

```
0.05|00013⟩ + 0.08|00022⟩ + 0.05|00031⟩ + 0.05|00103⟩ + 0.14|00112⟩ + 0.14|00121⟩ + 0.05|00130⟩ + 0.08|00202⟩ + 0.14|
```

```
n=5
k=5
# 0 < k < 3n
qr = cirq.LineQid.range(n, dimension=4)
test=cirq.Circuit(spin32Dicke(qr,n,k))
#print(test)
result = simulator.simulate(test)
print(cirq.dirac_notation(result.final_state_vector, qid_shape=(4,)*n))
```

```
0.07|10013⟩ + 0.12|10022⟩ + 0.07|10031⟩ + 0.07|10103⟩ + 0.2|10112⟩ + 0.2|10121⟩ + 0.07|10130⟩ + 0.12|10202⟩ + 0.2|102
```

```
n=5
k=6
# 0 < k < 3n
qr = cirq.LineQid.range(n, dimension=4)
test=cirq.Circuit(spin32Dicke(qr,n,k))
#print(test)
result = simulator.simulate(test)
print(cirq.dirac_notation(result.final_state_vector, qid_shape=(4,)*n))
```

```
0.01|00033⟩ + 0.04|00123⟩ + 0.04|00132⟩ + 0.04|00213⟩ + 0.07|00222⟩ + 0.04|00231⟩ + 0.01|00303⟩ + 0.04|00312⟩ + 0.04|
```

```
n=5
k=7
# 0 < k < 3n
qr = cirq.LineQid.range(n, dimension=4)
test=cirq.Circuit(spin32Dicke(qr,n,k))
#print(test)
result = simulator.simulate(test)
print(cirq.dirac_notation(result.final_state_vector, qid_shape=(4,)*n))
```

```
0.02|00133⟩ + 0.04|00223⟩ + 0.04|00232⟩ + 0.02|00313⟩ + 0.04|00322⟩ + 0.02|00331⟩ + 0.02|01033⟩ + 0.06|01123⟩ + 0.06|
```

```
n=5
k=8
# 0 < k < 3n
qr = cirq.LineQid.range(n, dimension=4)
test=cirq.Circuit(spin32Dicke(qr,n,k))
#print(test)
result = simulator.simulate(test)
print(cirq.dirac_notation(result.final_state_vector, qid_shape=(4,)*n))
```

```
0.02|00233⟩ + 0.02|00323⟩ + 0.02|00332⟩ + 0.04|01133⟩ + 0.06|01223⟩ + 0.06|01232⟩ + 0.04|01313⟩ + 0.06|01322⟩ + 0.04|
```

```
n=5
k=9
# 0 < k < 3n
qr = cirq.LineQid.range(n, dimension=4)
test=cirq.Circuit(spin32Dicke(qr,n,k))
#print(test)
result = simulator.simulate(test)
print(cirq.dirac_notation(result.final_state_vector, qid_shape=(4,)*n))
```

```
0.01|00333⟩ + 0.04|01233⟩ + 0.04|01323⟩ + 0.04|01332⟩ + 0.04|02133⟩ + 0.07|02223⟩ + 0.07|02232⟩ + 0.04|02313⟩ + 0.07|
```

## Simplified

For $m \leq n$,

$$\mathcal{W}_{m,k}^{(3/2)} = \prod_{k'=max(k-3(n-m),1)}^{min(k,3m-1)} T_{m,k'}^{(3/2)}$$

```
def mystate(qr,n,k):
  """Gives generator"""
  # initial state
  l=round(np.floor(k/3))
  if k==3*l:
    for j in range(l):
      yield X03()(qr[j])

  elif k==3*l+1:
    for j in range(l):
      yield X03()(qr[j])
    yield X01()(qr[l])

  elif k==3*l+2:
    for j in range(l):
      yield X03()(qr[j])
    yield X02()(qr[l])


def Wnew(qr,m,k):
  for kp in range(max(k-3*(n-m),1),min(k,3*m-1)+1):
    yield t_gate(qr,m,kp)

#W \otimes identity:
def WWnew(qr,n,m,k):
  yield Wnew(qr[n-m:n],m,k)

def UUnew(qr,n,k):
  for m in reversed(range(2,n+1)):
    yield WWnew(qr,n,m,k)

def spin32DickeNew(qr,n,k):
  """Gives generator"""
  # 0 < k < 3n
  # initial state
  yield mystate(qr,n,k)
  # apply Dicke operator
  yield UUnew(qr,n,k)
```

## n=2

```
n=2
k=1
# 0 < k < 3n
qr = cirq.LineQid.range(n, dimension=4)
test=cirq.Circuit(spin32DickeNew(qr,n,k))
#print(test)
result = simulator.simulate(test)
print(cirq.dirac_notation(result.final_state_vector, qid_shape=(4,)*n))
```

```
0.71|01⟩ + 0.71|10⟩
```

```
test=cirq.Circuit(spin32Dicke(qr,n,k))
#print(test)
result = simulator.simulate(test)
print(cirq.dirac_notation(result.final_state_vector, qid_shape=(4,)*n))
```

```
0.71|01⟩ + 0.71|10⟩
```

```
n=2
k=2
# 0 < k < 3n
qr = cirq.LineQid.range(n, dimension=4)
test=cirq.Circuit(spin32DickeNew(qr,n,k))
#print(test)
result = simulator.simulate(test)
print(cirq.dirac_notation(result.final_state_vector, qid_shape=(4,)*n))
```

```
0.45|02⟩ + 0.77|11⟩ + 0.45|20⟩
```

```
test=cirq.Circuit(spin32Dicke(qr,n,k))
#print(test)
result = simulator.simulate(test)
print(cirq.dirac_notation(result.final_state_vector, qid_shape=(4,)*n))
```

```
0.45|02⟩ + 0.77|11⟩ + 0.45|20⟩
```

```
n=2
k=3
# 0 < k < 3n
qr = cirq.LineQid.range(n, dimension=4)
test=cirq.Circuit(spin32DickeNew(qr,n,k))
#print(test)
result = simulator.simulate(test)
print(cirq.dirac_notation(result.final_state_vector, qid_shape=(4,)*n))
```

```
0.22|03⟩ + 0.67|12⟩ + 0.67|21⟩ + 0.22|30⟩
```

```
test=cirq.Circuit(spin32Dicke(qr,n,k))
#print(test)
result = simulator.simulate(test)
print(cirq.dirac_notation(result.final_state_vector, qid_shape=(4,)*n))
```

```
0.22|03⟩ + 0.67|12⟩ + 0.67|21⟩ + 0.22|30⟩
```

```
n=2
k=4
# 0 < k < 3n
qr = cirq.LineQid.range(n, dimension=4)
test=cirq.Circuit(spin32DickeNew(qr,n,k))
#print(test)
result = simulator.simulate(test)
print(cirq.dirac_notation(result.final_state_vector, qid_shape=(4,)*n))
```

```
0.45|13⟩ + 0.77|22⟩ + 0.45|31⟩
```

```
test=cirq.Circuit(spin32Dicke(qr,n,k))
#print(test)
result = simulator.simulate(test)
print(cirq.dirac_notation(result.final_state_vector, qid_shape=(4,)*n))
```

```
0.45|13⟩ + 0.77|22⟩ + 0.45|31⟩
```

```
n=2
k=5
# 0 < k < 3n
qr = cirq.LineQid.range(n, dimension=4)
test=cirq.Circuit(spin32DickeNew(qr,n,k))
#print(test)
result = simulator.simulate(test)
print(cirq.dirac_notation(result.final_state_vector, qid_shape=(4,)*n))
```

```
0.71|23⟩ + 0.71|32⟩
```

```
test=cirq.Circuit(spin32Dicke(qr,n,k))
#print(test)
result = simulator.simulate(test)
```
