# Supplementary material for: Spin-s Dicke states and their preparation
Source: arXiv:2402.03233 source file (2024-08-18)
Supplement: Supplementary file 2 [file s=1_Dicke_arxiv.pdf]

# Spin-1 Dicke states

```
try:
    import cirq
except ImportError:
    print("installing cirq...")
    !pip install --quiet cirq
    import cirq

    print("installed cirq.")
```

## Basic qutrit gates

```
import numpy as np
```

```
simulator = cirq.Simulator()
```

```
class X01(cirq.Gate):

  def _qid_shape_(self):
    return (3,)

  def _unitary_(self):
    return np.array([[0, 1, 0],
                    [1, 0, 0],
                    [0, 0, 1]])

  def _circuit_diagram_info_(self, args):
        return 'X01'

class X02(cirq.Gate):

  def _qid_shape_(self):
    return (3,)

  def _unitary_(self):
    return np.array([[0, 0, 1],
                    [0, 1, 0],
                    [1, 0, 0]])

  def _circuit_diagram_info_(self, args):
        return 'X02'

class X12(cirq.Gate):

  def _qid_shape_(self):
    return (3,)

  def _unitary_(self):
    return np.array([[1, 0, 0],
                    [0, 0, 1],
                    [0, 1, 0]])

  def _circuit_diagram_info_(self, args):
        return 'X12'

class R01(cirq.Gate):

  def __init__(self, theta):
        super(R01, self)
        self.theta = theta

  def _qid_shape_(self):
    return (3,)

  def _unitary_(self):
    return np.array([[np.cos(self.theta/2), -np.sin(self.theta/2), 0],
                    [np.sin(self.theta/2), np.cos(self.theta/2), 0],
                    [0, 0, 1]])

  def _circuit_diagram_info_(self, args):
        return f"R01({self.theta})"

class R02(cirq.Gate):

  def __init__(self, theta):
        super(R02, self)
        self.theta = theta

  def _qid_shape_(self):
    return (3,)

  def _unitary_(self):
    return np.array([[np.cos(self.theta/2), 0, -np.sin(self.theta/2)],
                     [0, 1, 0],
                     [np.sin(self.theta/2), 0, np.cos(self.theta/2)]
                    ])

  def _circuit_diagram_info_(self, args):
        return f"R02({self.theta})"

class R12(cirq.Gate):

  def __init__(self, theta):
```

```
        super(R12, self)
        self.theta = theta

  def _qid_shape_(self):
    return (3,)

  def _unitary_(self):
    return np.array([[1, 0, 0],
                     [0, np.cos(self.theta/2), -np.sin(self.theta/2)],
                     [0, np.sin(self.theta/2), np.cos(self.theta/2)]
                      ])

  def _circuit_diagram_info_(self, args):
        return f"R12({self.theta})"


class myid(cirq.Gate):

  def _qid_shape_(self):
    return (3,)

  def _unitary_(self):
    return np.array([[1, 0, 0],
                    [0, 1, 0],
                    [0, 0, 1]])

  def _circuit_diagram_info_(self, args):
        return 'id'
```

## T operators

$$T_{m,k} (1 \leq k \leq 2n-1)$$

```
# even

# k = 2l even, 2 \le l \le m-1 , m \ge 3
def t_gate0_a(qr,m,l):
  """Gives generator"""
  # l=k/2
  k=2*l
  cx12 = cirq.ControlledGate(X12(),num_controls=1, control_values=(1,),\
                             control_qid_shape=(3,))
  cx01 = cirq.ControlledGate(X01(),num_controls=1, control_values=(2,),\
                             control_qid_shape=(3,))


  theta1=-2*np.arccos(np.sqrt((k*(k-1))/(2*m*(2*m-1))))
  theta2=-2*np.arctan(np.sqrt((2*m-k-1)/(2*k)))

  ccr12 = cirq.ControlledGate(R12(theta1),num_controls=2, \
                              control_values=((1,),(2,)),\
                              control_qid_shape=(3,3))
  ccr01 = cirq.ControlledGate(R01(theta2),num_controls=2, \
                              control_values=((2,),(2,)),\
                              control_qid_shape=(3,3))

  yield cx01(qr[0],qr[l])
  yield ccr12(qr[l],qr[l-1],qr[0])
  yield cx01(qr[0],qr[l])

  yield cx12(qr[0],qr[l])
  yield ccr01(qr[l],qr[l-1],qr[0])
  yield cx12(qr[0],qr[l])

# k = 2l even, l=1, m \ge 2
def t_gate0_b(qr,m,l):
  """Gives generator"""
  # l=1
  k=2*l
  cx12 = cirq.ControlledGate(X12(),num_controls=1, control_values=(1,),\
                             control_qid_shape=(3,))
  cx01 = cirq.ControlledGate(X01(),num_controls=1, control_values=(2,),\
                             control_qid_shape=(3,))

  theta1=-2*np.arccos(np.sqrt((k*(k-1))/(2*m*(2*m-1))))
  theta2=-2*np.arctan(np.sqrt((2*m-k-1)/(2*k)))

  cr12 = cirq.ControlledGate(R12(theta1),num_controls=1, \
                              control_values=(1,),\
                              control_qid_shape=(3,))
  cr01 = cirq.ControlledGate(R01(theta2),num_controls=1, \
                              control_values=(2,),\
                              control_qid_shape=(3,))

  yield cx01(qr[0],qr[l])
  yield cr12(qr[l],qr[0])
  yield cx01(qr[0],qr[l])

  yield cx12(qr[0],qr[l])
  yield cr01(qr[l],qr[0])
  yield cx12(qr[0],qr[l])

# odd

# k = 2l+1 odd, 2 \le l \le m-2 , m \ge 4
def t_gate1_a(qr,m,l):
  """Gives generator"""
  k=2*l+1
  cx12 = cirq.ControlledGate(X12(),num_controls=1, control_values=(2,),\
                             control_qid_shape=(3,))
  cx01 = cirq.ControlledGate(X01(),num_controls=1, control_values=(1,),\
                             control_qid_shape=(3,))

  theta1=-2*np.arccos(np.sqrt((k*(k-1))/(2*m*(2*m-1))))
  theta2=-2*np.arctan(np.sqrt((2*m-k-1)/(2*k)))

  ccr12 = cirq.ControlledGate(R12(theta1),num_controls=2, \
                              control_values=((2,),(2,)),\
                              control_qid_shape=(3,3))
  ccr01 = cirq.ControlledGate(R01(theta2),num_controls=2, \
```

```
                            control_values=((1,),(2,)),\
                            control_qid_shape=(3,3))

  yield cx12(qr[0],qr[l])
  yield ccr12(qr[l],qr[l-1],qr[0])
  yield cx12(qr[0],qr[l])
  yield cx01(qr[0],qr[l+1])
  yield ccr01(qr[l+1],qr[l],qr[0])
  yield cx01(qr[0],qr[l+1])


# k = 2l+1 odd, l= m-1 , m \ge 3
def t_gate1_b(qr,m,l):
  """Gives generator"""
  # l=m-1
  k=2*l+1
  cx12 = cirq.ControlledGate(X12(),num_controls=1, control_values=(2,),\
                           control_qid_shape=(3,))
  cx01 = cirq.ControlledGate(X01(),num_controls=1, control_values=(1,),\
                           control_qid_shape=(3,))

  theta1=-2*np.arccos(np.sqrt(((k-1))/(2*m)))

  ccr12 = cirq.ControlledGate(R12(theta1),num_controls=2, \
                            control_values=((2,),(2,)),\
                            control_qid_shape=(3,3))

  yield cx12(qr[0],qr[l])
  yield ccr12(qr[l],qr[l-1],qr[0])
  yield cx12(qr[0],qr[l])


# k = 2l+1 odd, l=1, m=2
def t_gate1_c(qr,m,l):
  """Gives generator"""
  # m=2
  # l=1
  k=2*l+1
  cx12 = cirq.ControlledGate(X12(),num_controls=1, control_values=(2,),\
                           control_qid_shape=(3,))

  theta1=-2*np.arccos(np.sqrt(3/(m*(2*m-1))))

  cr12 = cirq.ControlledGate(R12(theta1),num_controls=1, \
                            control_values=(2,),\
                            control_qid_shape=(3,))

  yield cx12(qr[0],qr[l])
  yield cr12(qr[l],qr[0])
  yield cx12(qr[0],qr[l])


# k = 2l+1 odd, l=1 , m \ge 3
def t_gate1_d(qr,m,l):
  """Gives generator"""
  # l=1
  k=2*l+1
  cx12 = cirq.ControlledGate(X12(),num_controls=1, control_values=(2,),\
                           control_qid_shape=(3,))
  cx01 = cirq.ControlledGate(X01(),num_controls=1, control_values=(1,),\
                           control_qid_shape=(3,))

  theta1=-2*np.arccos(np.sqrt(3/(m*(2*m-1))))
  theta2=-2*np.arctan(np.sqrt((m-2)/3))

  cr12 = cirq.ControlledGate(R12(theta1),num_controls=1, \
                            control_values=(2,),\
                            control_qid_shape=(3,))
  ccr01 = cirq.ControlledGate(R01(theta2),num_controls=2, \
                            control_values=((1,),(2,)),\
                            control_qid_shape=(3,3))

  yield cx12(qr[0],qr[l])
  yield cr12(qr[l],qr[0])
  yield cx12(qr[0],qr[l])
  yield cx01(qr[0],qr[l+1])
  yield ccr01(qr[l+1],qr[l],qr[0])
```

```
  yield cx01(qr[0],qr[l+1])


# k = 2l+1 odd, l=0 , m \ge 2
def t_gate1_e(qr,m,l):
  """Gives generator"""
  # l=0
  k=2*l+1
  cx01 = cirq.ControlledGate(X01(),num_controls=1, control_values=(1,),\
                           control_qid_shape=(3,))

  theta2=-2*np.arctan(np.sqrt(m-1))

  cr01 = cirq.ControlledGate(R01(theta2),num_controls=1, \
                            control_values=(1,),\
                            control_qid_shape=(3,))

  yield cx01(qr[0],qr[l+1])
  yield cr01(qr[l+1],qr[0])
  yield cx01(qr[0],qr[l+1])


def t_gate(qr,m,k):
  l=round(np.floor(k/2))
  if k==2*l:
     mycase=0
  elif k==2*l+1:
     mycase=1

  if mycase==0 and 2 <= l <= m-1 and m>=3:
    yield t_gate0_a(qr,m,l)

  elif mycase==0 and l==1 and m>=2:
    yield t_gate0_b(qr,m,l)

  elif mycase==1 and 2 <= l <= m-2 and m>=4:
    yield t_gate1_a(qr,m,l)

  elif mycase==1 and l== m-1 and m>=3:
    yield t_gate1_b(qr,m,l)

  elif mycase==1 and l== 1 and m==2:
    yield t_gate1_c(qr,m,l)

  elif mycase==1 and l== 1 and m>=3:
    yield t_gate1_d(qr,m,l)

  elif mycase==1 and l== 0 and m>=2:
    yield t_gate1_e(qr,m,l)
```

## Reference state

```
def mystate(qr,n,k):
  """Gives generator"""
  # initial state
  l=round(np.floor(k/2))
  if k==2*l:
    for j in range(l):
      yield X02()(qr[j])
    for j in range(l,n):
      yield myid()(qr[j])
  elif k==2*l+1:
    for j in range(l):
      yield X02()(qr[j])
    yield X01()(qr[l])
    for j in range(l,n):
      yield myid()(qr[j])
```

## NOT simplified

```
def W(qr,m):
  for k in range(1,2*m):
    yield t_gate(qr,m,k)

#W \otimes identity:
def WW(qr,n,m):
  yield W(qr[n-m:n],m)

def UU(qr,n):
  for m in reversed(range(2,n+1)):
    yield WW(qr,n,m)

def spin1Dicke(qr,n,k):
  """Gives generator"""
  # 0 < k < 2n
  # initial state
  yield mystate(qr,n,k)
  # apply Dicke operator
  yield UU(qr,n)
```

## n=2

```
n=2
k=1
# 0 < k < 2n
qr = cirq.LineQid.range(n, dimension=3)
test=cirq.Circuit(spin1Dicke(qr,n,k))
#print(test)
result = simulator.simulate(test)
print(cirq.dirac_notation(result.final_state_vector, qid_shape=(3,)*n))
```

```
0.71|01⟩ + 0.71|10⟩
```

```
n=2
k=2
# 0 < k < 2n
qr = cirq.LineQid.range(n, dimension=3)
test=cirq.Circuit(spin1Dicke(qr,n,k))
#print(test)
result = simulator.simulate(test)
print(cirq.dirac_notation(result.final_state_vector, qid_shape=(3,)*n))
```

```
0.41|02⟩ + 0.82|11⟩ + 0.41|20⟩
```

```
n=2
k=3
# 0 < k < 2n
qr = cirq.LineQid.range(n, dimension=3)
test=cirq.Circuit(spin1Dicke(qr,n,k))
#print(test)
result = simulator.simulate(test)
print(cirq.dirac_notation(result.final_state_vector, qid_shape=(3,)*n))
```

```
0.71|12⟩ + 0.71|21⟩
```

## n=3

```
n=3
k=1
# 0 < k < 2n
qr = cirq.LineQid.range(n, dimension=3)
test=cirq.Circuit(spin1Dicke(qr,n,k))
#print(test)
result = simulator.simulate(test)
print(cirq.dirac_notation(result.final_state_vector, qid_shape=(3,)*n))
```

```
0.58|001⟩ + 0.58|010⟩ + 0.58|100⟩
```

```
n=3
k=2
# 0 < k < 2n
qr = cirq.LineQid.range(n, dimension=3)
test=cirq.Circuit(spin1Dicke(qr,n,k))
#print(test)
result = simulator.simulate(test)
print(cirq.dirac_notation(result.final_state_vector, qid_shape=(3,)*n))
```

```
0.26|002⟩ + 0.52|011⟩ + 0.26|020⟩ + 0.52|101⟩ + 0.52|110⟩ + 0.26|200⟩
```

```
n=3
k=3
# 0 < k < 2n
qr = cirq.LineQid.range(n, dimension=3)
test=cirq.Circuit(spin1Dicke(qr,n,k))
#print(test)
result = simulator.simulate(test)
print(cirq.dirac_notation(result.final_state_vector, qid_shape=(3,)*n))
```

```
0.32|012⟩ + 0.32|021⟩ + 0.32|102⟩ + 0.63|111⟩ + 0.32|120⟩ + 0.32|201⟩ + 0.32|210⟩
```

```
n=3
k=4
# 0 < k < 2n
qr = cirq.LineQid.range(n, dimension=3)
test=cirq.Circuit(spin1Dicke(qr,n,k))
#print(test)
result = simulator.simulate(test)
print(cirq.dirac_notation(result.final_state_vector, qid_shape=(3,)*n))
```

```
0.26|022⟩ + 0.52|112⟩ + 0.52|121⟩ + 0.26|202⟩ + 0.52|211⟩ + 0.26|220⟩
```

```
n=3
k=5
# 0 < k < 2n
qr = cirq.LineQid.range(n, dimension=3)
test=cirq.Circuit(spin1Dicke(qr,n,k))
#print(test)
result = simulator.simulate(test)
print(cirq.dirac_notation(result.final_state_vector, qid_shape=(3,)*n))
```

```
0.58|122⟩ + 0.58|212⟩ + 0.58|221⟩
```

## n=4

```
n=4
k=1
# 0 < k < 2n
qr = cirq.LineQid.range(n, dimension=3)
test=cirq.Circuit(spin1Dicke(qr,n,k))
#print(test)
result = simulator.simulate(test)
print(cirq.dirac_notation(result.final_state_vector, qid_shape=(3,)*n))
```

```
0.5|0001⟩ + 0.5|0010⟩ + 0.5|0100⟩ + 0.5|1000⟩
```

```
n=4
k=2
# 0 < k < 2n
qr = cirq.LineQid.range(n, dimension=3)
test=cirq.Circuit(spin1Dicke(qr,n,k))
#print(test)
result = simulator.simulate(test)
print(cirq.dirac_notation(result.final_state_vector, qid_shape=(3,)*n))
```

```
0.19|0002⟩ + 0.38|0011⟩ + 0.19|0020⟩ + 0.38|0101⟩ + 0.38|0110⟩ + 0.19|0200⟩ + 0.38|1001⟩ + 0.38|1010⟩ + 0.38|1100⟩ + 0.19|2000⟩
```

```
n=4
k=3
# 0 < k < 2n
qr = cirq.LineQid.range(n, dimension=3)
test=cirq.Circuit(spin1Dicke(qr,n,k))
#print(test)
result = simulator.simulate(test)
print(cirq.dirac_notation(result.final_state_vector, qid_shape=(3,)*n))
```

```
0.19|0012⟩ + 0.19|0021⟩ + 0.19|0102⟩ + 0.38|0111⟩ + 0.19|0120⟩ + 0.19|0201⟩ + 0.19|0210⟩ + 0.19|1002⟩ + 0.38|1011⟩ + 0.19|1020⟩ + 0.38|1101
```

```
n=4
k=4
# 0 < k < 2n
qr = cirq.LineQid.range(n, dimension=3)
test=cirq.Circuit(spin1Dicke(qr,n,k))
#print(test)
result = simulator.simulate(test)
print(cirq.dirac_notation(result.final_state_vector, qid_shape=(3,)*n))
```

```
0.12|0022⟩ + 0.24|0112⟩ + 0.24|0121⟩ + 0.12|0202⟩ + 0.24|0211⟩ + 0.12|0220⟩ + 0.24|1012⟩ + 0.24|1021⟩ + 0.24|1102⟩ + 0.48|1111⟩ + 0.24|1120
```

```
n=4
k=5
# 0 < k < 2n
qr = cirq.LineQid.range(n, dimension=3)
test=cirq.Circuit(spin1Dicke(qr,n,k))
#print(test)
result = simulator.simulate(test)
print(cirq.dirac_notation(result.final_state_vector, qid_shape=(3,)*n))
```

```
0.19|0122⟩ + 0.19|0212⟩ + 0.19|0221⟩ + 0.19|1022⟩ + 0.38|1112⟩ + 0.38|1121⟩ + 0.19|1202⟩ + 0.38|1211⟩ + 0.19|1220⟩ + 0.19|2012⟩ + 0.19|2021
```

```
n=4
k=6
# 0 < k < 2n
qr = cirq.LineQid.range(n, dimension=3)
test=cirq.Circuit(spin1Dicke(qr,n,k))
#print(test)
result = simulator.simulate(test)
print(cirq.dirac_notation(result.final_state_vector, qid_shape=(3,)*n))
```

```
0.19|0222⟩ + 0.38|1122⟩ + 0.38|1212⟩ + 0.38|1221⟩ + 0.19|2022⟩ + 0.38|2112⟩ + 0.38|2121⟩ + 0.19|2202⟩ + 0.38|2211⟩ + 0.19|2220⟩
```

```
n=4
k=7
# 0 < k < 2n
qr = cirq.LineQid.range(n, dimension=3)
test=cirq.Circuit(spin1Dicke(qr,n,k))
#print(test)
result = simulator.simulate(test)
print(cirq.dirac_notation(result.final_state_vector, qid_shape=(3,)*n))
```

```
0.5|1222⟩ + 0.5|2122⟩ + 0.5|2212⟩ + 0.5|2221⟩
```

## n=5

```
n=5
k=1
# 0 < k < 2n
qr = cirq.LineQid.range(n, dimension=3)
test=cirq.Circuit(spin1Dicke(qr,n,k))
#print(test)
result = simulator.simulate(test)
print(cirq.dirac_notation(result.final_state_vector, qid_shape=(3,)*n))
```

```
0.45|00001⟩ + 0.45|00010⟩ + 0.45|00100⟩ + 0.45|01000⟩ + 0.45|10000⟩
```

```
n=5
k=2
# 0 < k < 2n
qr = cirq.LineQid.range(n, dimension=3)
test=cirq.Circuit(spin1Dicke(qr,n,k))
#print(test)
result = simulator.simulate(test)
print(cirq.dirac_notation(result.final_state_vector, qid_shape=(3,)*n))
```

```
0.15|00002⟩ + 0.3|00011⟩ + 0.15|00020⟩ + 0.3|00101⟩ + 0.3|00110⟩ + 0.15|00200⟩ + 0.3|01001⟩ + 0.3|01010⟩ + 0.3|01100⟩ + 0.15|02000⟩ + 0.3|1
```

```
n=5
k=3
# 0 < k < 2n
qr = cirq.LineQid.range(n, dimension=3)
test=cirq.Circuit(spin1Dicke(qr,n,k))
#print(test)
result = simulator.simulate(test)
print(cirq.dirac_notation(result.final_state_vector, qid_shape=(3,)*n))
```

```
0.13|00012⟩ + 0.13|00021⟩ + 0.13|00102⟩ + 0.26|00111⟩ + 0.13|00120⟩ + 0.13|00201⟩ + 0.13|00210⟩ + 0.13|01002⟩ + 0.26|01011⟩ + 0.13|01020⟩ +
```

```
n=5
k=4
# 0 < k < 2n
qr = cirq.LineQid.range(n, dimension=3)
test=cirq.Circuit(spin1Dicke(qr,n,k))
#print(test)
result = simulator.simulate(test)
print(cirq.dirac_notation(result.final_state_vector, qid_shape=(3,)*n))
```

```
0.07|00022⟩ + 0.14|00112⟩ + 0.14|00121⟩ + 0.07|00202⟩ + 0.14|00211⟩ + 0.07|00220⟩ + 0.14|01012⟩ + 0.14|01021⟩ + 0.14|01102⟩ + 0.28|01111⟩ +
```

```
n=5
k=5
# 0 < k < 2n
qr = cirq.LineQid.range(n, dimension=3)
test=cirq.Circuit(spin1Dicke(qr,n,k))
#print(test)
result = simulator.simulate(test)
print(cirq.dirac_notation(result.final_state_vector, qid_shape=(3,)*n))
```

```
0.09|00122⟩ + 0.09|00212⟩ + 0.09|00221⟩ + 0.09|01022⟩ + 0.18|01112⟩ + 0.18|01121⟩ + 0.09|01202⟩ + 0.18|01211⟩ + 0.09|01220⟩ + 0.09|02012⟩ +
```

```
n=5
k=6
# 0 < k < 2n
qr = cirq.LineQid.range(n, dimension=3)
test=cirq.Circuit(spin1Dicke(qr,n,k))
#print(test)
result = simulator.simulate(test)
print(cirq.dirac_notation(result.final_state_vector, qid_shape=(3,)*n))
```

```
0.07|00222⟩ + 0.14|01122⟩ + 0.14|01212⟩ + 0.14|01221⟩ + 0.07|02022⟩ + 0.14|02112⟩ + 0.14|02121⟩ + 0.07|02202⟩ + 0.14|02211⟩ + 0.07|02220⟩ +
```

```
n=5
k=7
# 0 < k < 2n
qr = cirq.LineQid.range(n, dimension=3)
test=cirq.Circuit(spin1Dicke(qr,n,k))
#print(test)
result = simulator.simulate(test)
print(cirq.dirac_notation(result.final_state_vector, qid_shape=(3,)*n))
```

```
0.13|01222⟩ + 0.13|02122⟩ + 0.13|02212⟩ + 0.13|02221⟩ + 0.13|10222⟩ + 0.26|11122⟩ + 0.26|11212⟩ + 0.26|11221⟩ + 0.13|12022⟩ + 0.26|12112⟩ +
```

```
n=5
k=8
# 0 < k < 2n
qr = cirq.LineQid.range(n, dimension=3)
test=cirq.Circuit(spin1Dicke(qr,n,k))
#print(test)
result = simulator.simulate(test)
print(cirq.dirac_notation(result.final_state_vector, qid_shape=(3,)*n))
```

```
0.15|02222⟩ + 0.3|11222⟩ + 0.3|12122⟩ + 0.3|12212⟩ + 0.3|12221⟩ + 0.15|20222⟩ + 0.3|21122⟩ + 0.3|21212⟩ + 0.3|21221⟩ + 0.15|22022⟩ + 0.3|22
```

```
n=5
k=9
# 0 < k < 2n
qr = cirq.LineQid.range(n, dimension=3)
test=cirq.Circuit(spin1Dicke(qr,n,k))
#print(test)
result = simulator.simulate(test)
print(cirq.dirac_notation(result.final_state_vector, qid_shape=(3,)*n))
```

```
0.45|12222⟩ + 0.45|21222⟩ + 0.45|22122⟩ + 0.45|22212⟩ + 0.45|22221⟩
```

## n=6

```
n=6
k=1
# 0 < k < 2n
qr = cirq.LineQid.range(n, dimension=3)
test=cirq.Circuit(spin1Dicke(qr,n,k))
#print(test)
result = simulator.simulate(test)
print(cirq.dirac_notation(result.final_state_vector, qid_shape=(3,)*n))
```

```
0.41|000001⟩ + 0.41|000010⟩ + 0.41|000100⟩ + 0.41|001000⟩ + 0.41|010000⟩ + 0.41|100000⟩
```

```
n=6
k=2
# 0 < k < 2n
qr = cirq.LineQid.range(n, dimension=3)
test=cirq.Circuit(spin1Dicke(qr,n,k))
#print(test)
result = simulator.simulate(test)
print(cirq.dirac_notation(result.final_state_vector, qid_shape=(3,)*n))
```

```
0.12|000002⟩ + 0.25|000011⟩ + 0.12|000020⟩ + 0.25|000101⟩ + 0.25|000110⟩ + 0.12|000200⟩ + 0.25|001001⟩ + 0.25|001010⟩ + 0.25|001100⟩ + 0.12
```

```
n=6
k=3
# 0 < k < 2n
qr = cirq.LineQid.range(n, dimension=3)
test=cirq.Circuit(spin1Dicke(qr,n,k))
#print(test)
result = simulator.simulate(test)
print(cirq.dirac_notation(result.final_state_vector, qid_shape=(3,)*n))
```

```
0.1|000012⟩ + 0.1|000021⟩ + 0.1|000102⟩ + 0.19|000111⟩ + 0.1|000120⟩ + 0.1|000201⟩ + 0.1|000210⟩ + 0.1|001002⟩ + 0.19|001011⟩ + 0.1|001020⟩
```

```
n=6
k=4
# 0 < k < 2n
qr = cirq.LineQid.range(n, dimension=3)
test=cirq.Circuit(spin1Dicke(qr,n,k))
#print(test)
result = simulator.simulate(test)
print(cirq.dirac_notation(result.final_state_vector, qid_shape=(3,)*n))
```

```
0.04|000022⟩ + 0.09|000112⟩ + 0.09|000121⟩ + 0.04|000202⟩ + 0.09|000211⟩ + 0.04|000220⟩ + 0.09|001012⟩ + 0.09|001021⟩ + 0.09|001102⟩ + 0.18
```

```
n=6
k=5
# 0 < k < 2n
qr = cirq.LineQid.range(n, dimension=3)
test=cirq.Circuit(spin1Dicke(qr,n,k))
#print(test)
result = simulator.simulate(test)
print(cirq.dirac_notation(result.final_state_vector, qid_shape=(3,)*n))
```

```
0.05|000122⟩ + 0.05|000212⟩ + 0.05|000221⟩ + 0.05|001022⟩ + 0.1|001112⟩ + 0.1|001121⟩ + 0.05|001202⟩ + 0.1|001211⟩ + 0.05|001220⟩ + 0.05|00
```

```
n=6
k=6
# 0 < k < 2n
qr = cirq.LineQid.range(n, dimension=3)
test=cirq.Circuit(spin1Dicke(qr,n,k))
#print(test)
result = simulator.simulate(test)
print(cirq.dirac_notation(result.final_state_vector, qid_shape=(3,)*n))
```

```
0.03|000222⟩ + 0.07|001122⟩ + 0.07|001212⟩ + 0.07|001221⟩ + 0.03|002022⟩ + 0.07|002112⟩ + 0.07|002121⟩ + 0.03|002202⟩ + 0.07|002211⟩ + 0.03
```

```
n=6
k=7
# 0 < k < 2n
qr = cirq.LineQid.range(n, dimension=3)
test=cirq.Circuit(spin1Dicke(qr,n,k))
#print(test)
result = simulator.simulate(test)
print(cirq.dirac_notation(result.final_state_vector, qid_shape=(3,)*n))
```

```
0.05|001222⟩ + 0.05|002122⟩ + 0.05|002212⟩ + 0.05|002221⟩ + 0.05|010222⟩ + 0.1|011122⟩ + 0.1|011212⟩ + 0.1|011221⟩ + 0.05|012022⟩ + 0.1|012
```

```
n=6
k=8
# 0 < k < 2n
qr = cirq.LineQid.range(n, dimension=3)
test=cirq.Circuit(spin1Dicke(qr,n,k))
#print(test)
result = simulator.simulate(test)
print(cirq.dirac_notation(result.final_state_vector, qid_shape=(3,)*n))
```

```
0.04|002222⟩ + 0.09|011222⟩ + 0.09|012122⟩ + 0.09|012212⟩ + 0.09|012221⟩ + 0.04|020222⟩ + 0.09|021122⟩ + 0.09|021212⟩ + 0.09|021221⟩ + 0.04
```

```
n=6
k=9
# 0 < k < 2n
qr = cirq.LineQid.range(n, dimension=3)
test=cirq.Circuit(spin1Dicke(qr,n,k))
#print(test)
result = simulator.simulate(test)
print(cirq.dirac_notation(result.final_state_vector, qid_shape=(3,)*n))
```

```
0.1|012222⟩ + 0.1|021222⟩ + 0.1|022122⟩ + 0.1|022212⟩ + 0.1|022221⟩ + 0.1|102222⟩ + 0.19|111222⟩ + 0.19|112122⟩ + 0.19|112212⟩ + 0.19|11222
```

```
n=6
k=10
# 0 < k < 2n
qr = cirq.LineQid.range(n, dimension=3)
test=cirq.Circuit(spin1Dicke(qr,n,k))
#print(test)
result = simulator.simulate(test)
print(cirq.dirac_notation(result.final_state_vector, qid_shape=(3,)*n))
```

```
0.12|022222⟩ + 0.25|112222⟩ + 0.25|121222⟩ + 0.25|122122⟩ + 0.25|122212⟩ + 0.25|122221⟩ + 0.12|202222⟩ + 0.25|211222⟩ + 0.25|212122⟩ + 0.25
```

```
n=6
k=11
# 0 < k < 2n
qr = cirq.LineQid.range(n, dimension=3)
test=cirq.Circuit(spin1Dicke(qr,n,k))
#print(test)
result = simulator.simulate(test)
print(cirq.dirac_notation(result.final_state_vector, qid_shape=(3,)*n))
```

```
0.41|122222⟩ + 0.41|212222⟩ + 0.41|221222⟩ + 0.41|222122⟩ + 0.41|222212⟩ + 0.41|222221⟩
```

## Simplified

For $m \leq n$,

$$\mathcal{W}^{(1)}_{m,k} = \prod_{k'=max(k-2(n-m),1)}^{min(k,2m-1)} T^{(1)}_{m,k'}$$

```
def Wnew(qr,m,k):
  for kp in range(max(k-2*(n-m),1),min(k,2*m-1)+1):
    yield t_gate(qr,m,kp)

#W \otimes identity:
def WWnew(qr,n,m,k):
  yield Wnew(qr[n-m:n],m,k)

def UUnew(qr,n,k):
  for m in reversed(range(2,n+1)):
    yield WWnew(qr,n,m,k)

def spin1DickeNew(qr,n,k):
  """Gives generator"""
  # 0 < k < 2n
  # initial state
  yield mystate(qr,n,k)
  # apply Dicke operator
  yield UUnew(qr,n,k)
```

## n=2

```
n=2
k=1
# 0 < k < 2n
qr = cirq.LineQid.range(n, dimension=3)
test=cirq.Circuit(spin1Dicke(qr,n,k))
#print(test)
result = simulator.simulate(test)
print(cirq.dirac_notation(result.final_state_vector, qid_shape=(3,)*n))
```

```
0.71|01⟩ + 0.71|10⟩
```

```
test=cirq.Circuit(spin1DickeNew(qr,n,k))
#print(test)
result = simulator.simulate(test)
print(cirq.dirac_notation(result.final_state_vector, qid_shape=(3,)*n))
```

```
0.71|01⟩ + 0.71|10⟩
```

```
n=2
k=2
# 0 < k < 2n
qr = cirq.LineQid.range(n, dimension=3)
test=cirq.Circuit(spin1Dicke(qr,n,k))
#print(test)
result = simulator.simulate(test)
print(cirq.dirac_notation(result.final_state_vector, qid_shape=(3,)*n))
```

```
0.41|02⟩ + 0.82|11⟩ + 0.41|20⟩
```

```
test=cirq.Circuit(spin1DickeNew(qr,n,k))
#print(test)
result = simulator.simulate(test)
print(cirq.dirac_notation(result.final_state_vector, qid_shape=(3,)*n))
```

    0.41|02⟩ + 0.82|11⟩ + 0.41|20⟩

```
n=2
k=3
# 0 < k < 2n
qr = cirq.LineQid.range(n, dimension=3)
test=cirq.Circuit(spin1Dicke(qr,n,k))
#print(test)
result = simulator.simulate(test)
print(cirq.dirac_notation(result.final_state_vector, qid_shape=(3,)*n))
```

    0.71|12⟩ + 0.71|21⟩

```
test=cirq.Circuit(spin1DickeNew(qr,n,k))
#print(test)
result = simulator.simulate(test)
print(cirq.dirac_notation(result.final_state_vector, qid_shape=(3,)*n))
```

    0.71|12⟩ + 0.71|21⟩

## n=3

```
n=3
k=1
# 0 < k < 2n
qr = cirq.LineQid.range(n, dimension=3)
test=cirq.Circuit(spin1Dicke(qr,n,k))
#print(test)
result = simulator.simulate(test)
print(cirq.dirac_notation(result.final_state_vector, qid_shape=(3,)*n))
```

    0.58|001⟩ + 0.58|010⟩ + 0.58|100⟩

```
test=cirq.Circuit(spin1DickeNew(qr,n,k))
#print(test)
result = simulator.simulate(test)
print(cirq.dirac_notation(result.final_state_vector, qid_shape=(3,)*n))
```

    0.58|001⟩ + 0.58|010⟩ + 0.58|100⟩

```
n=3
k=2
# 0 < k < 2n
qr = cirq.LineQid.range(n, dimension=3)
test=cirq.Circuit(spin1Dicke(qr,n,k))
#print(test)
result = simulator.simulate(test)
print(cirq.dirac_notation(result.final_state_vector, qid_shape=(3,)*n))
```

    0.26|002⟩ + 0.52|011⟩ + 0.26|020⟩ + 0.52|101⟩ + 0.52|110⟩ + 0.26|200⟩

```
test=cirq.Circuit(spin1DickeNew(qr,n,k))
#print(test)
result = simulator.simulate(test)
print(cirq.dirac_notation(result.final_state_vector, qid_shape=(3,)*n))
```

    0.26|002⟩ + 0.52|011⟩ + 0.26|020⟩ + 0.52|101⟩ + 0.52|110⟩ + 0.26|200⟩

```
n=3
k=3
# 0 < k < 2n
qr = cirq.LineQid.range(n, dimension=3)
test=cirq.Circuit(spin1Dicke(qr,n,k))
#print(test)
result = simulator.simulate(test)
print(cirq.dirac_notation(result.final_state_vector, qid_shape=(3,)*n))
```

```
0.32|012⟩ + 0.32|021⟩ + 0.32|102⟩ + 0.63|111⟩ + 0.32|120⟩ + 0.32|201⟩ + 0.32|210⟩
```

```
test=cirq.Circuit(spin1DickeNew(qr,n,k))
#print(test)
result = simulator.simulate(test)
print(cirq.dirac_notation(result.final_state_vector, qid_shape=(3,)*n))
```

```
0.32|012⟩ + 0.32|021⟩ + 0.32|102⟩ + 0.63|111⟩ + 0.32|120⟩ + 0.32|201⟩ + 0.32|210⟩
```

```
n=3
k=4
# 0 < k < 2n
qr = cirq.LineQid.range(n, dimension=3)
test=cirq.Circuit(spin1Dicke(qr,n,k))
#print(test)
result = simulator.simulate(test)
print(cirq.dirac_notation(result.final_state_vector, qid_shape=(3,)*n))
```

```
0.26|022⟩ + 0.52|112⟩ + 0.52|121⟩ + 0.26|202⟩ + 0.52|211⟩ + 0.26|220⟩
```

```
test=cirq.Circuit(spin1DickeNew(qr,n,k))
#print(test)
result = simulator.simulate(test)
print(cirq.dirac_notation(result.final_state_vector, qid_shape=(3,)*n))
```

```
0.26|022⟩ + 0.52|112⟩ + 0.52|121⟩ + 0.26|202⟩ + 0.52|211⟩ + 0.26|220⟩
```

```
n=3
k=5
# 0 < k < 2n
qr = cirq.LineQid.range(n, dimension=3)
test=cirq.Circuit(spin1Dicke(qr,n,k))
#print(test)
result = simulator.simulate(test)
print(cirq.dirac_notation(result.final_state_vector, qid_shape=(3,)*n))
```

```
0.58|122⟩ + 0.58|212⟩ + 0.58|221⟩
```

```
test=cirq.Circuit(spin1DickeNew(qr,n,k))
#print(test)
result = simulator.simulate(test)
print(cirq.dirac_notation(result.final_state_vector, qid_shape=(3,)*n))
```

```
0.58|122⟩ + 0.58|212⟩ + 0.58|221⟩
```

## n=4

```
n=4
k=1
# 0 < k < 2n
qr = cirq.LineQid.range(n, dimension=3)
test=cirq.Circuit(spin1Dicke(qr,n,k))
#print(test)
result = simulator.simulate(test)
print(cirq.dirac_notation(result.final_state_vector, qid_shape=(3,)*n))
```

```
0.5|0001⟩ + 0.5|0010⟩ + 0.5|0100⟩ + 0.5|1000⟩
```

```
test=cirq.Circuit(spin1DickeNew(qr,n,k))
#print(test)
result = simulator.simulate(test)
print(cirq.dirac_notation(result.final_state_vector, qid_shape=(3,)*n))
```

```
0.5|0001⟩ + 0.5|0010⟩ + 0.5|0100⟩ + 0.5|1000⟩
```

```
n=4
k=2
# 0 < k < 2n
qr = cirq.LineQid.range(n, dimension=3)
test=cirq.Circuit(spin1Dicke(qr,n,k))
#print(test)
result = simulator.simulate(test)
print(cirq.dirac_notation(result.final_state_vector, qid_shape=(3,)*n))
```

```
0.19|0002⟩ + 0.38|0011⟩ + 0.19|0020⟩ + 0.38|0101⟩ + 0.38|0110⟩ + 0.19|0200⟩ + 0.38|1001⟩ + 0.38|1010⟩ + 0.38|1100⟩ + 0.19|2000⟩
```

```
test=cirq.Circuit(spin1DickeNew(qr,n,k))
#print(test)
result = simulator.simulate(test)
print(cirq.dirac_notation(result.final_state_vector, qid_shape=(3,)*n))
```

```
0.19|0002⟩ + 0.38|0011⟩ + 0.19|0020⟩ + 0.38|0101⟩ + 0.38|0110⟩ + 0.19|0200⟩ + 0.38|1001⟩ + 0.38|1010⟩ + 0.38|1100⟩ + 0.19|2000⟩
```

```
n=4
k=3
# 0 < k < 2n
qr = cirq.LineQid.range(n, dimension=3)
test=cirq.Circuit(spin1Dicke(qr,n,k))
#print(test)
result = simulator.simulate(test)
print(cirq.dirac_notation(result.final_state_vector, qid_shape=(3,)*n))
```

```
0.19|0012⟩ + 0.19|0021⟩ + 0.19|0102⟩ + 0.38|0111⟩ + 0.19|0120⟩ + 0.19|0201⟩ + 0.19|0210⟩ + 0.19|1002⟩ + 0.38|1011⟩ + 0.19|1020⟩ + 0.38|1101
```

```
test=cirq.Circuit(spin1DickeNew(qr,n,k))
#print(test)
result = simulator.simulate(test)
print(cirq.dirac_notation(result.final_state_vector, qid_shape=(3,)*n))
```

```
0.19|0012⟩ + 0.19|0021⟩ + 0.19|0102⟩ + 0.38|0111⟩ + 0.19|0120⟩ + 0.19|0201⟩ + 0.19|0210⟩ + 0.19|1002⟩ + 0.38|1011⟩ + 0.19|1020⟩ + 0.38|1101
```

```
n=4
k=4
# 0 < k < 2n
qr = cirq.LineQid.range(n, dimension=3)
test=cirq.Circuit(spin1Dicke(qr,n,k))
#print(test)
result = simulator.simulate(test)
print(cirq.dirac_notation(result.final_state_vector, qid_shape=(3,)*n))
```

```
0.12|0022⟩ + 0.24|0112⟩ + 0.24|0121⟩ + 0.12|0202⟩ + 0.24|0211⟩ + 0.12|0220⟩ + 0.24|1012⟩ + 0.24|1021⟩ + 0.24|1102⟩ + 0.48|1111⟩ + 0.24|1120
```

```
test=cirq.Circuit(spin1DickeNew(qr,n,k))
#print(test)
result = simulator.simulate(test)
print(cirq.dirac_notation(result.final_state_vector, qid_shape=(3,)*n))
```

```
0.12|0022⟩ + 0.24|0112⟩ + 0.24|0121⟩ + 0.12|0202⟩ + 0.24|0211⟩ + 0.12|0220⟩ + 0.24|1012⟩ + 0.24|1021⟩ + 0.24|1102⟩ + 0.48|1111⟩ + 0.24|1120
```

```
n=4
k=5
# 0 < k < 2n
qr = cirq.LineQid.range(n, dimension=3)
test=cirq.Circuit(spin1Dicke(qr,n,k))
#print(test)
result = simulator.simulate(test)
print(cirq.dirac_notation(result.final_state_vector, qid_shape=(3,)*n))
```

```
0.19|0122⟩ + 0.19|0212⟩ + 0.19|0221⟩ + 0.19|1022⟩ + 0.38|1112⟩ + 0.38|1121⟩ + 0.19|1202⟩ + 0.38|1211⟩ + 0.19|1220⟩ + 0.19|2012⟩ + 0.19|2021
```

```
test=cirq.Circuit(spin1DickeNew(qr,n,k))
#print(test)
result = simulator.simulate(test)
print(cirq.dirac_notation(result.final_state_vector, qid_shape=(3,)*n))
```

```
0.19|0122⟩ + 0.19|0212⟩ + 0.19|0221⟩ + 0.19|1022⟩ + 0.38|1112⟩ + 0.38|1121⟩ + 0.19|1202⟩ + 0.38|1211⟩ + 0.19|1220⟩ + 0.19|2012⟩ + 0.19|2021
```

```
n=4
k=6
# 0 < k < 2n
qr = cirq.LineQid.range(n, dimension=3)
test=cirq.Circuit(spin1Dicke(qr,n,k))
#print(test)
result = simulator.simulate(test)
print(cirq.dirac_notation(result.final_state_vector, qid_shape=(3,)*n))
```

```
0.19|0222⟩ + 0.38|1122⟩ + 0.38|1212⟩ + 0.38|1221⟩ + 0.19|2022⟩ + 0.38|2112⟩ + 0.38|2121⟩ + 0.19|2202⟩ + 0.38|2211⟩ + 0.19|2220⟩
```

```
test=cirq.Circuit(spin1DickeNew(qr,n,k))
#print(test)
result = simulator.simulate(test)
print(cirq.dirac_notation(result.final_state_vector, qid_shape=(3,)*n))
```

```
0.19|0222⟩ + 0.38|1122⟩ + 0.38|1212⟩ + 0.38|1221⟩ + 0.19|2022⟩ + 0.38|2112⟩ + 0.38|2121⟩ + 0.19|2202⟩ + 0.38|2211⟩ + 0.19|2220⟩
```

```
n=4
k=7
# 0 < k < 2n
qr = cirq.LineQid.range(n, dimension=3)
test=cirq.Circuit(spin1Dicke(qr,n,k))
#print(test)
result = simulator.simulate(test)
print(cirq.dirac_notation(result.final_state_vector, qid_shape=(3,)*n))
```

```
0.5|1222⟩ + 0.5|2122⟩ + 0.5|2212⟩ + 0.5|2221⟩
```

```
test=cirq.Circuit(spin1DickeNew(qr,n,k))
#print(test)
result = simulator.simulate(test)
print(cirq.dirac_notation(result.final_state_vector, qid_shape=(3,)*n))
```

```
0.5|1222⟩ + 0.5|2122⟩ + 0.5|2212⟩ + 0.5|2221⟩
```

## n=5

```
n=5
k=1
# 0 < k < 2n
qr = cirq.LineQid.range(n, dimension=3)
test=cirq.Circuit(spin1Dicke(qr,n,k))
#print(test)
result = simulator.simulate(test)
print(cirq.dirac_notation(result.final_state_vector, qid_shape=(3,)*n))
```

```
0.45|00001⟩ + 0.45|00010⟩ + 0.45|00100⟩ + 0.45|01000⟩ + 0.45|10000⟩
```

```
test=cirq.Circuit(spin1DickeNew(qr,n,k))
#print(test)
result = simulator.simulate(test)
print(cirq.dirac_notation(result.final_state_vector, qid_shape=(3,)*n))
```

```
0.45|00001⟩ + 0.45|00010⟩ + 0.45|00100⟩ + 0.45|01000⟩ + 0.45|10000⟩
```

```
n=5
k=2
# 0 < k < 2n
qr = cirq.LineQid.range(n, dimension=3)
test=cirq.Circuit(spin1Dicke(qr,n,k))
#print(test)
result = simulator.simulate(test)
print(cirq.dirac_notation(result.final_state_vector, qid_shape=(3,)*n))
```

```
0.15|00002⟩ + 0.3|00011⟩ + 0.15|00020⟩ + 0.3|00101⟩ + 0.3|00110⟩ + 0.15|00200⟩ + 0.3|01001⟩ + 0.3|01010⟩ + 0.3|01100⟩ + 0.15|02000⟩ + 0.3|1
```

```
test=cirq.Circuit(spin1DickeNew(qr,n,k))
#print(test)
result = simulator.simulate(test)
print(cirq.dirac_notation(result.final_state_vector, qid_shape=(3,)*n))
```

```
0.15|00002⟩ + 0.3|00011⟩ + 0.15|00020⟩ + 0.3|00101⟩ + 0.3|00110⟩ + 0.15|00200⟩ + 0.3|01001⟩ + 0.3|01010⟩ + 0.3|01100⟩ + 0.15|02000⟩ + 0.3|1
```

```
n=5
k=3
# 0 < k < 2n
qr = cirq.LineQid.range(n, dimension=3)
test=cirq.Circuit(spin1Dicke(qr,n,k))
#print(test)
result = simulator.simulate(test)
print(cirq.dirac_notation(result.final_state_vector, qid_shape=(3,)*n))
```

```
0.13|00012⟩ + 0.13|00021⟩ + 0.13|00102⟩ + 0.26|00111⟩ + 0.13|00120⟩ + 0.13|00201⟩ + 0.13|00210⟩ + 0.13|01002⟩ + 0.26|01011⟩ + 0.13|01020⟩ +
```

```
test=cirq.Circuit(spin1DickeNew(qr,n,k))
#print(test)
result = simulator.simulate(test)
print(cirq.dirac_notation(result.final_state_vector, qid_shape=(3,)*n))
```

```
0.13|00012⟩ + 0.13|00021⟩ + 0.13|00102⟩ + 0.26|00111⟩ + 0.13|00120⟩ + 0.13|00201⟩ + 0.13|00210⟩ + 0.13|01002⟩ + 0.26|01011⟩ + 0.13|01020⟩ +
```

```
n=5
k=4
# 0 < k < 2n
qr = cirq.LineQid.range(n, dimension=3)
test=cirq.Circuit(spin1Dicke(qr,n,k))
#print(test)
result = simulator.simulate(test)
print(cirq.dirac_notation(result.final_state_vector, qid_shape=(3,)*n))
```

```
0.07|00022⟩ + 0.14|00112⟩ + 0.14|00121⟩ + 0.07|00202⟩ + 0.14|00211⟩ + 0.07|00220⟩ + 0.14|01012⟩ + 0.14|01021⟩ + 0.14|01102⟩ + 0.28|01111⟩ +
```

```
test=cirq.Circuit(spin1DickeNew(qr,n,k))
#print(test)
result = simulator.simulate(test)
print(cirq.dirac_notation(result.final_state_vector, qid_shape=(3,)*n))
```

```
0.07|00022⟩ + 0.14|00112⟩ + 0.14|00121⟩ + 0.07|00202⟩ + 0.14|00211⟩ + 0.07|00220⟩ + 0.14|01012⟩ + 0.14|01021⟩ + 0.14|01102⟩ + 0.28|01111⟩ +
```

```
n=5
k=5
# 0 < k < 2n
qr = cirq.LineQid.range(n, dimension=3)
test=cirq.Circuit(spin1Dicke(qr,n,k))
#print(test)
result = simulator.simulate(test)
print(cirq.dirac_notation(result.final_state_vector, qid_shape=(3,)*n))
```

```
0.09|00122⟩ + 0.09|00212⟩ + 0.09|00221⟩ + 0.09|01022⟩ + 0.18|01112⟩ + 0.18|01121⟩ + 0.09|01202⟩ + 0.18|01211⟩ + 0.09|01220⟩ + 0.09|02012⟩ +
```

```
test=cirq.Circuit(spin1DickeNew(qr,n,k))
#print(test)
result = simulator.simulate(test)
print(cirq.dirac_notation(result.final_state_vector, qid_shape=(3,)*n))
```

```
0.09|00122⟩ + 0.09|00212⟩ + 0.09|00221⟩ + 0.09|01022⟩ + 0.18|01112⟩ + 0.18|01121⟩ + 0.09|01202⟩ + 0.18|01211⟩ + 0.09|01220⟩ + 0.09|02012⟩ +
```

```
n=5
k=5
# 0 < k < 2n
qr = cirq.LineQid.range(n, dimension=3)
test=cirq.Circuit(spin1Dicke(qr,n,k))
#print(test)
result = simulator.simulate(test)
print(cirq.dirac_notation(result.final_state_vector, qid_shape=(3,)*n))
```

```
0.09|00122⟩ + 0.09|00212⟩ + 0.09|00221⟩ + 0.09|01022⟩ + 0.18|01112⟩ + 0.18|01121⟩ + 0.09|01202⟩ + 0.18|01211⟩ + 0.09|01220⟩ + 0.09|02012⟩ +
```

```
test=cirq.Circuit(spin1DickeNew(qr,n,k))
#print(test)
result = simulator.simulate(test)
print(cirq.dirac_notation(result.final_state_vector, qid_shape=(3,)*n))
```

```
0.09|00122⟩ + 0.09|00212⟩ + 0.09|00221⟩ + 0.09|01022⟩ + 0.18|01112⟩ + 0.18|01121⟩ + 0.09|01202⟩ + 0.18|01211⟩ + 0.09|01220⟩ + 0.09|02012⟩ +
```

```
n=5
k=6
# 0 < k < 2n
qr = cirq.LineQid.range(n, dimension=3)
test=cirq.Circuit(spin1Dicke(qr,n,k))
#print(test)
result = simulator.simulate(test)
print(cirq.dirac_notation(result.final_state_vector, qid_shape=(3,)*n))
```

```
0.07|00222⟩ + 0.14|01122⟩ + 0.14|01212⟩ + 0.14|01221⟩ + 0.07|02022⟩ + 0.14|02112⟩ + 0.14|02121⟩ + 0.07|02202⟩ + 0.14|02211⟩ + 0.07|02220⟩ +
```

```
test=cirq.Circuit(spin1DickeNew(qr,n,k))
#print(test)
result = simulator.simulate(test)
print(cirq.dirac_notation(result.final_state_vector, qid_shape=(3,)*n))
```

```
0.07|00222⟩ + 0.14|01122⟩ + 0.14|01212⟩ + 0.14|01221⟩ + 0.07|02022⟩ + 0.14|02112⟩ + 0.14|02121⟩ + 0.07|02202⟩ + 0.14|02211⟩ + 0.07|02220⟩ +
```

```
n=5
k=7
# 0 < k < 2n
qr = cirq.LineQid.range(n, dimension=3)
test=cirq.Circuit(spin1Dicke(qr,n,k))
#print(test)
result = simulator.simulate(test)
print(cirq.dirac_notation(result.final_state_vector, qid_shape=(3,)*n))
```

```
0.13|01222⟩ + 0.13|02122⟩ + 0.13|02212⟩ + 0.13|02221⟩ + 0.13|10222⟩ + 0.26|11122⟩ + 0.26|11212⟩ + 0.26|11221⟩ + 0.13|12022⟩ + 0.26|12112⟩ +
```

```
test=cirq.Circuit(spin1DickeNew(qr,n,k))
#print(test)
result = simulator.simulate(test)
print(cirq.dirac_notation(result.final_state_vector, qid_shape=(3,)*n))
```

```
0.13|01222⟩ + 0.13|02122⟩ + 0.13|02212⟩ + 0.13|02221⟩ + 0.13|10222⟩ + 0.26|11122⟩ + 0.26|11212⟩ + 0.26|11221⟩ + 0.13|12022⟩ + 0.26|12112⟩ +
```

```
n=5
k=8
# 0 < k < 2n
qr = cirq.LineQid.range(n, dimension=3)
test=cirq.Circuit(spin1Dicke(qr,n,k))
#print(test)
```

```
test=cirq.Circuit(spin1DickeNew(qr,n,k))
#print(test)
result = simulator.simulate(test)
print(cirq.dirac_notation(result.final_state_vector, qid_shape=(3,)*n))
```

```
0.15|02222⟩ + 0.3|11222⟩ + 0.3|12122⟩ + 0.3|12212⟩ + 0.3|12221⟩ + 0.15|20222⟩ + 0.3|21122⟩ + 0.3|21212⟩ + 0.3|21221⟩ + 0.15|22022⟩ + 0.3|22
```

```
n=5
k=9
# 0 < k < 2n
qr = cirq.LineQid.range(n, dimension=3)
test=cirq.Circuit(spin1Dicke(qr,n,k))
#print(test)
result = simulator.simulate(test)
print(cirq.dirac_notation(result.final_state_vector, qid_shape=(3,)*n))
```

```
0.45|12222⟩ + 0.45|21222⟩ + 0.45|22122⟩ + 0.45|22212⟩ + 0.45|22221⟩
```

```
test=cirq.Circuit(spin1DickeNew(qr,n,k))
#print(test)
result = simulator.simulate(test)
print(cirq.dirac_notation(result.final_state_vector, qid_shape=(3,)*n))
```

```
0.45|12222⟩ + 0.45|21222⟩ + 0.45|22122⟩ + 0.45|22212⟩ + 0.45|22221⟩
```

## n=6

```
n=6
k=1
# 0 < k < 2n
qr = cirq.LineQid.range(n, dimension=3)
test=cirq.Circuit(spin1Dicke(qr,n,k))
#print(test)
result = simulator.simulate(test)
print(cirq.dirac_notation(result.final_state_vector, qid_shape=(3,)*n))
```

```
0.41|000001⟩ + 0.41|000010⟩ + 0.41|000100⟩ + 0.41|001000⟩ + 0.41|010000⟩ + 0.41|100000⟩
```

```
test=cirq.Circuit(spin1DickeNew(qr,n,k))
#print(test)
result = simulator.simulate(test)
print(cirq.dirac_notation(result.final_state_vector, qid_shape=(3,)*n))
```

```
0.41|000001⟩ + 0.41|000010⟩ + 0.41|000100⟩ + 0.41|001000⟩ + 0.41|010000⟩ + 0.41|100000⟩
```

```
n=6
k=2
# 0 < k < 2n
qr = cirq.LineQid.range(n, dimension=3)
test=cirq.Circuit(spin1Dicke(qr,n,k))
#print(test)
result = simulator.simulate(test)
print(cirq.dirac_notation(result.final_state_vector, qid_shape=(3,)*n))
```

```
0.12|000002⟩ + 0.25|000011⟩ + 0.12|000020⟩ + 0.25|000101⟩ + 0.25|000110⟩ + 0.12|000200⟩ + 0.25|001001⟩ + 0.25|001010⟩ + 0.25|001100⟩ + 0.12
```

```
test=cirq.Circuit(spin1DickeNew(qr,n,k))
#print(test)
result = simulator.simulate(test)
print(cirq.dirac_notation(result.final_state_vector, qid_shape=(3,)*n))
```
